# Supplementary material for: Stress-controlled medium-amplitude oscillatory shear (MAOStress) of PVA-Borax
Source: arXiv:2402.19357 source file (2024-02-29)
Supplement: Supplementary file 1 [file supp.tex]

\setcounter{figure}{0}

\section{Assessing the goodness of fit using the adjusted coefficient of determination}
The MAOStress material functions are defined based on the expansion of the strain harmonics in Eq. 4(a)-(d) up to first-order. These expressions fit the harmonics for most of the frequencies tested in this work. However, these expressions did not work well for very high and very low frequencies, especially for sub-dominant harmonics. In the viscous limit, the elastic harmonics are sub-dominant, which makes them noisy and causes them to deviate from the MAOS expansion. The viscous harmonics are subdominant in the elastic limit and suffer from the noise issue.

We use the adjusted coefficient of determination $R_{adj}^2$ to decide which data should be discarded systematically. This coefficient, computed using the statsmodel python package\cite{Seabold2010Statsmodels:Python}, quantifies the fraction of the data variability that is explained by the model ($0<R^2_{adj}<1$). We set the threshold to be 0.9, and any fit with less $R^2_{adj}$ will be discarded. Figure \ref{fig:3MAOSRadj} shows the coefficient for the four harmonics in Eq.4 as a function of frequency. 
\begin{figure}[h!]
   \centering
 \includegraphics{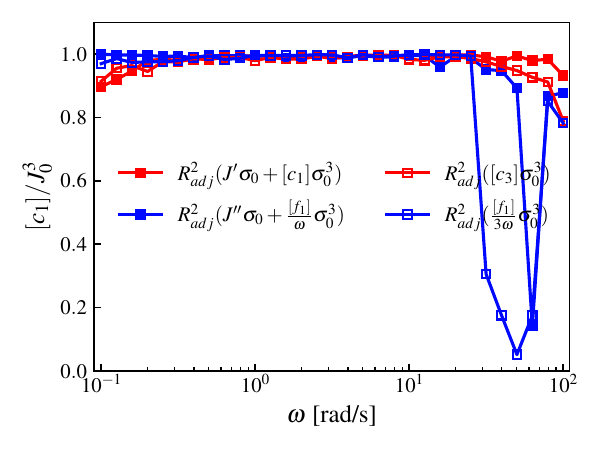}%
 \caption{The adjusted coefficient of determination $R^2_{adj}$ for the fits of experimental strain harmonics to Eq. 4(a)-(d). Each of the four harmonics has a different $R^2_{adj}$. Fits that have $R^2_{adj}<0.9$ are discarded.}
 \label{fig:3MAOSRadj}%
 \end{figure}
\section{Fits of MAOStress signals for all measured frequencies}
In this section, we include the primary data used to extract the MAOStress material functions of PVA-Borax, because extracting these material functions is not trivial. The power-law of 3 ($\sigma_0^3$) exhibited by the weakly nonlinear deviations in Eq. 4 does not hold for all materials \cite{Natalia2020QuestioningExpansions}. Moreoever, the fit should be restricted to the MAOS regime, which requires care in choosing where the MAOS regime starts and ends. In this work, we chose the limits of the MAOS regime based on the region where the stress amplitude is above the noise floor and below where higher order terms starts affecting the harmonics (deviation from power-law of 3). Acknowledging the subjectivity of the choice, we report on Figures S2-S32 the regions that were chosen to fit all four MAOStress material functions. To show the validity of the power-law of 3 assumption at different frequencies, we show the individual amplitude sweeps of first harmonic (a) elastic compliance $J_1^{\prime}$ and (b) viscous compliance $J_1^{\prime\prime}$ and the first-harmonic (c) elastic nonlinear deviation $\gamma_1^{\prime}-J^{\prime}\sigma_0$ and (d) viscous nonlinear deviation $\gamma_1^{\prime\prime}-J^{\prime\prime}\sigma_0$ and the third-harmonic (e) elastic nonlinear deviation $\gamma_3^{\prime}$ and (f) viscous nonlinear deviation $\gamma_3^{\prime\prime}$ in Figures S2-S32. Moreover, we will show the fits for the first and third-harmonics with the associated adjusted coefficient of determination $R^2_{adj}$ for each of the four fits (first and third elastic and viscous strain harmonics) to the MAOS expansions. 
\begin{figure}[h!] 
\centering
\includegraphics{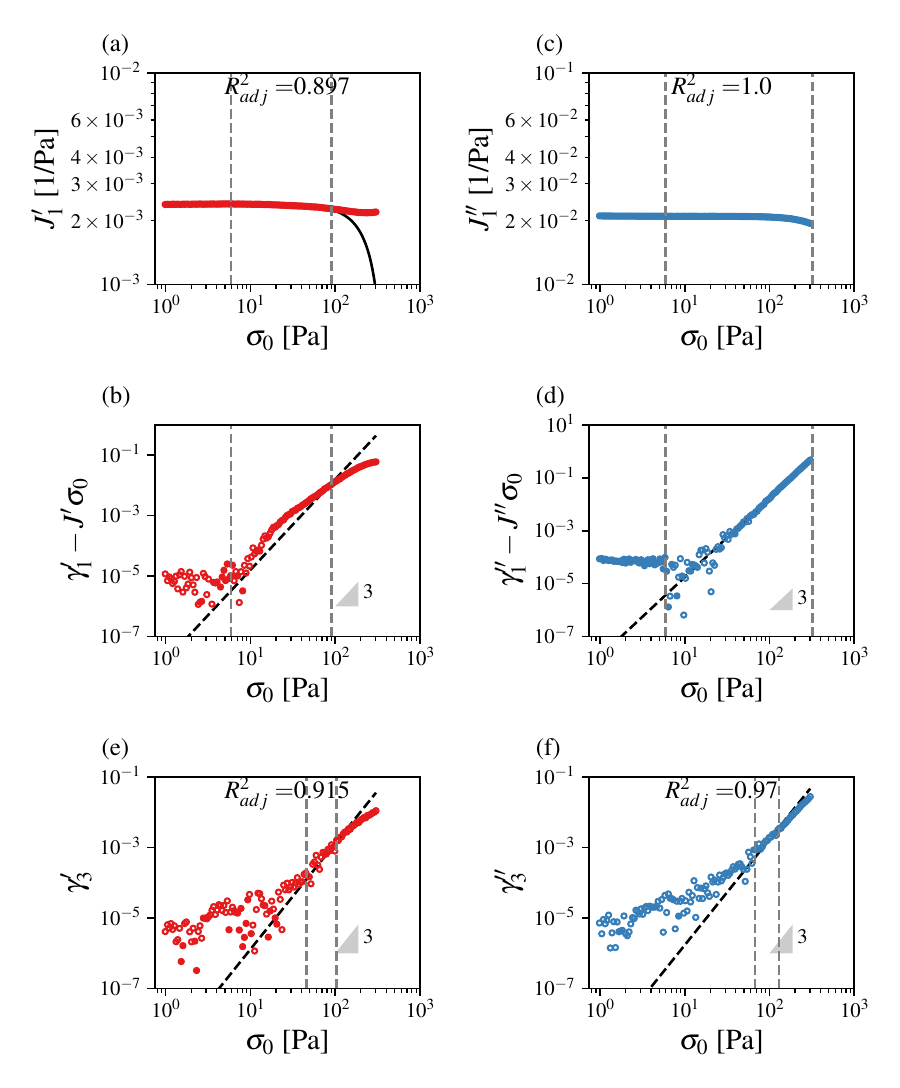}
\caption{The harmonics and fits for $\omega=0.1$ rad/s. Black lines are the fits to data using the MAOStress expansions in Eq. (4). Solid lines represent a positive sign  and dashed lines represent negative sign associated with the magnitude on the log-log scale. The gray vertical dashed lines represent the minimum and maximum stress amplitudes of the fit region that were chosen to fit the MAOStress expansion in Eq. (4).}
\end{figure}

\begin{figure}[h!] 
\centering
\includegraphics{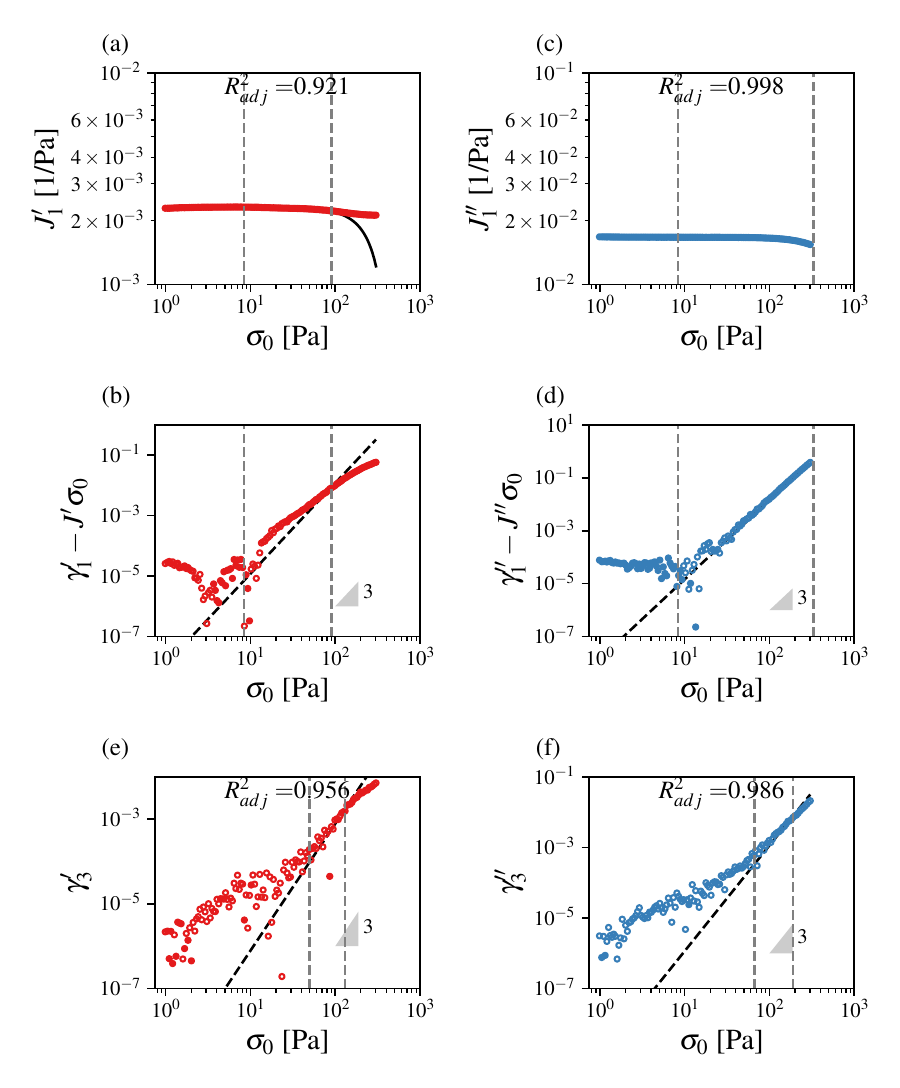}
\caption{The harmonics and fits for $\omega=0.126$ rad/s. Black lines are the fits to data using the MAOStress expansions in Eq. (4). Solid lines represent a positive sign  and dashed lines represent negative sign associated with the magnitude on the log-log scale. The gray vertical dashed lines represent the minimum and maximum stress amplitudes of the fit region that were chosen to fit the MAOStress expansion in Eq. (4).}
\end{figure}

\begin{figure}[h!] 
\centering
\includegraphics{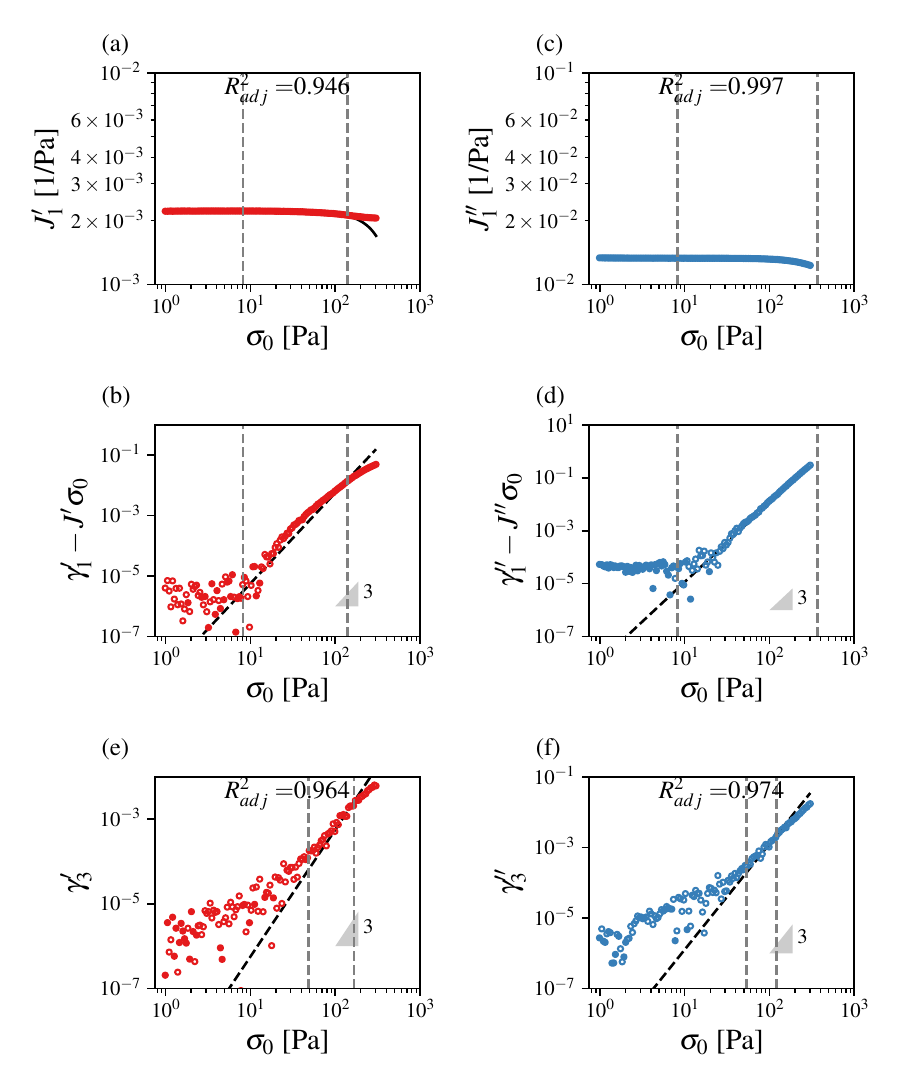}
\caption{The harmonics and fits for $\omega=0.158$ rad/s. Black lines are the fits to data using the MAOStress expansions in Eq. (4). Solid lines represent a positive sign  and dashed lines represent negative sign associated with the magnitude on the log-log scale. The gray vertical dashed lines represent the minimum and maximum stress amplitudes of the fit region that were chosen to fit the MAOStress expansion in Eq. (4).}
\end{figure}

\begin{figure}[h!] 
\centering
\includegraphics{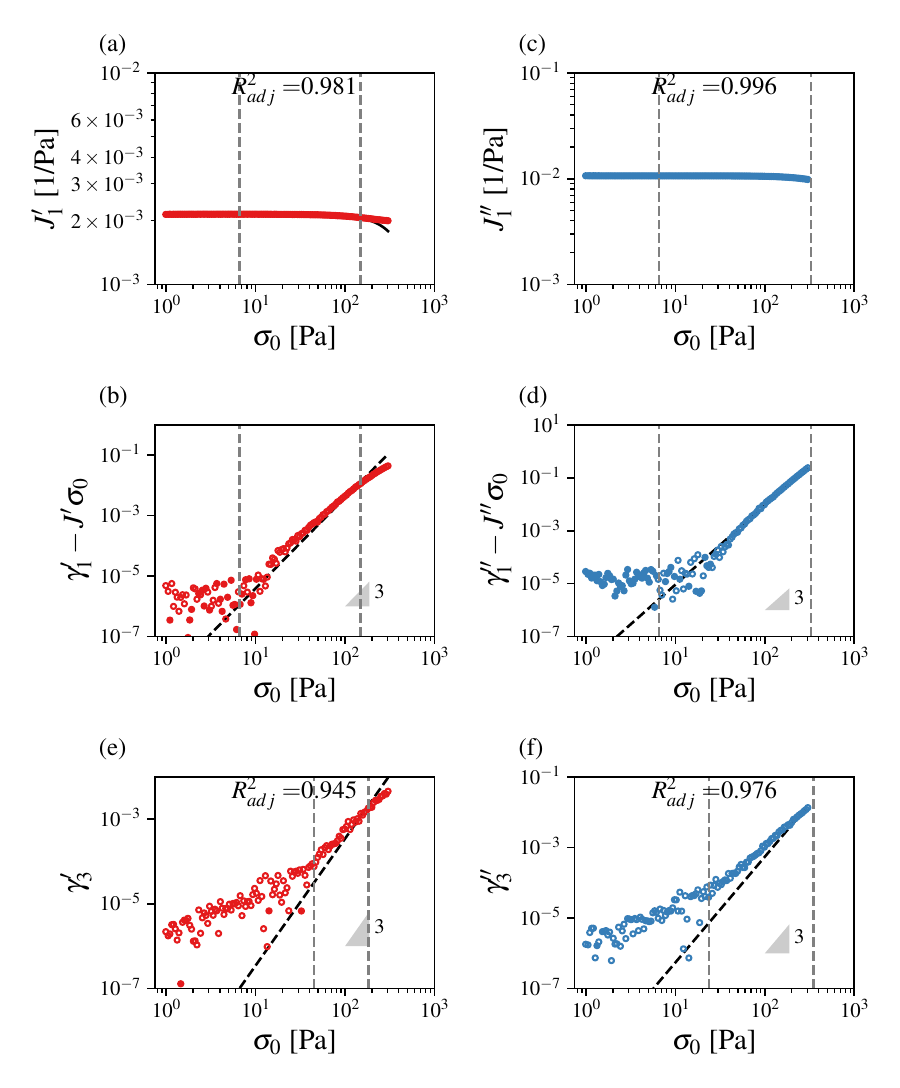}
\caption{The harmonics and fits for $\omega=0.2$ rad/s. Black lines are the fits to data using the MAOStress expansions in Eq. (4). Solid lines represent a positive sign  and dashed lines represent negative sign associated with the magnitude on the log-log scale. The gray vertical dashed lines represent the minimum and maximum stress amplitudes of the fit region that were chosen to fit the MAOStress expansion in Eq. (4).}
\end{figure}

\begin{figure}[h!] 
\centering
\includegraphics{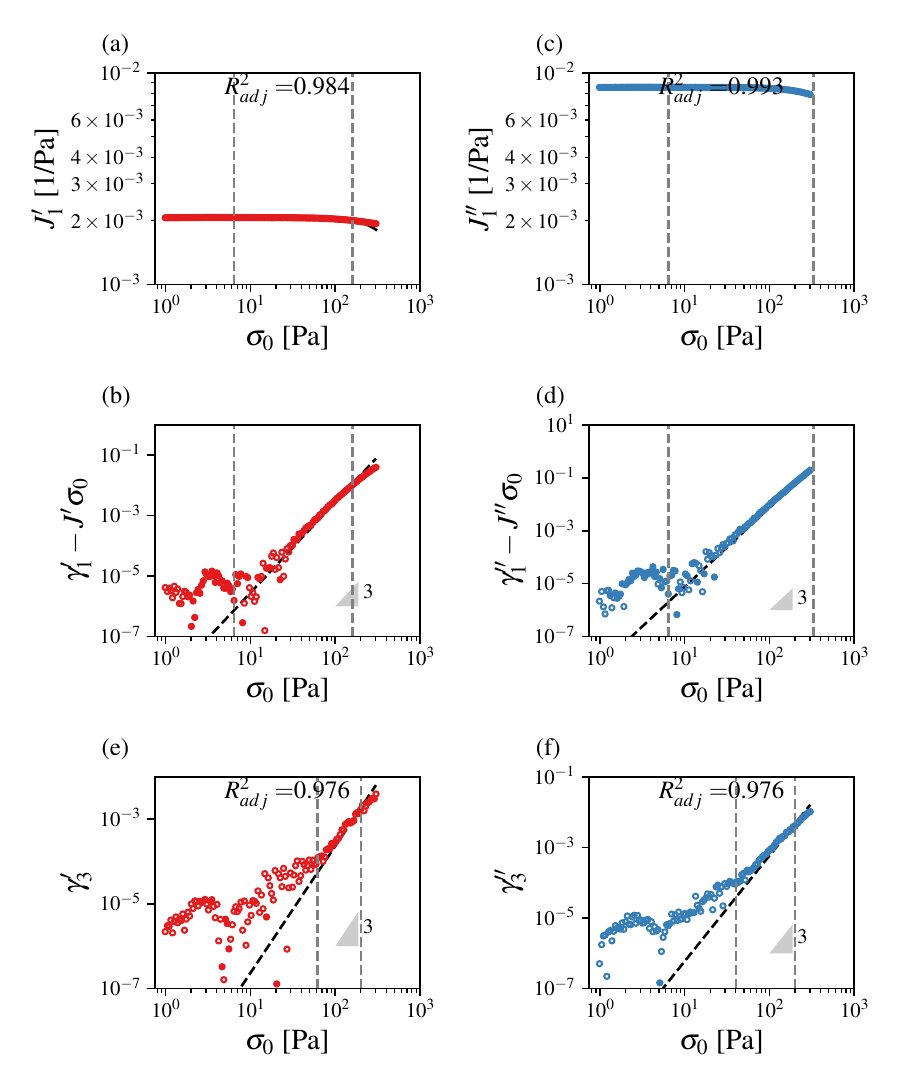}
\caption{The harmonics and fits for $\omega=0.251$ rad/s. Black lines are the fits to data using the MAOStress expansions in Eq. (4). Solid lines represent a positive sign  and dashed lines represent negative sign associated with the magnitude on the log-log scale. The gray vertical dashed lines represent the minimum and maximum stress amplitudes of the fit region that were chosen to fit the MAOStress expansion in Eq. (4).}
\end{figure}

\begin{figure}[h!] 
\centering
\includegraphics{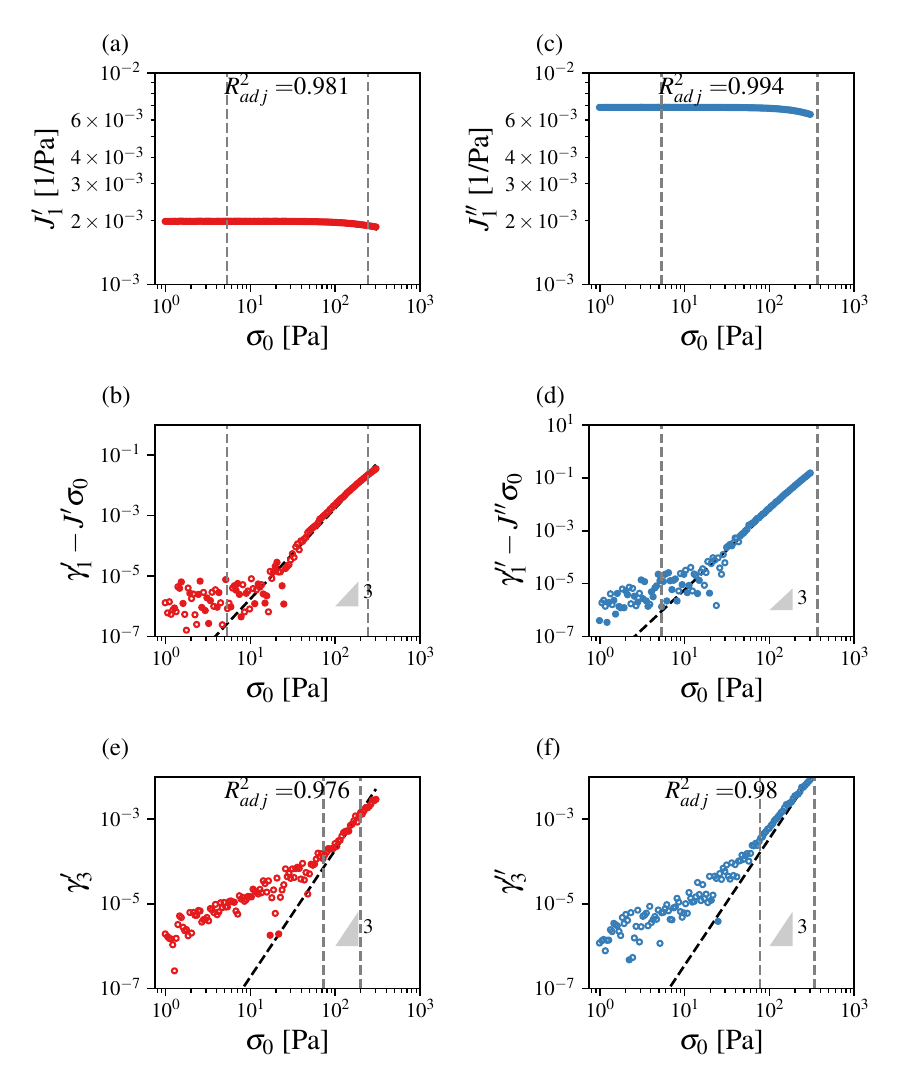}
\caption{The harmonics and fits for $\omega=0.316$ rad/s. Black lines are the fits to data using the MAOStress expansions in Eq. (4). Solid lines represent a positive sign  and dashed lines represent negative sign associated with the magnitude on the log-log scale. The gray vertical dashed lines represent the minimum and maximum stress amplitudes of the fit region that were chosen to fit the MAOStress expansion in Eq. (4).}
\end{figure}

\begin{figure}[h!] 
\centering
\includegraphics{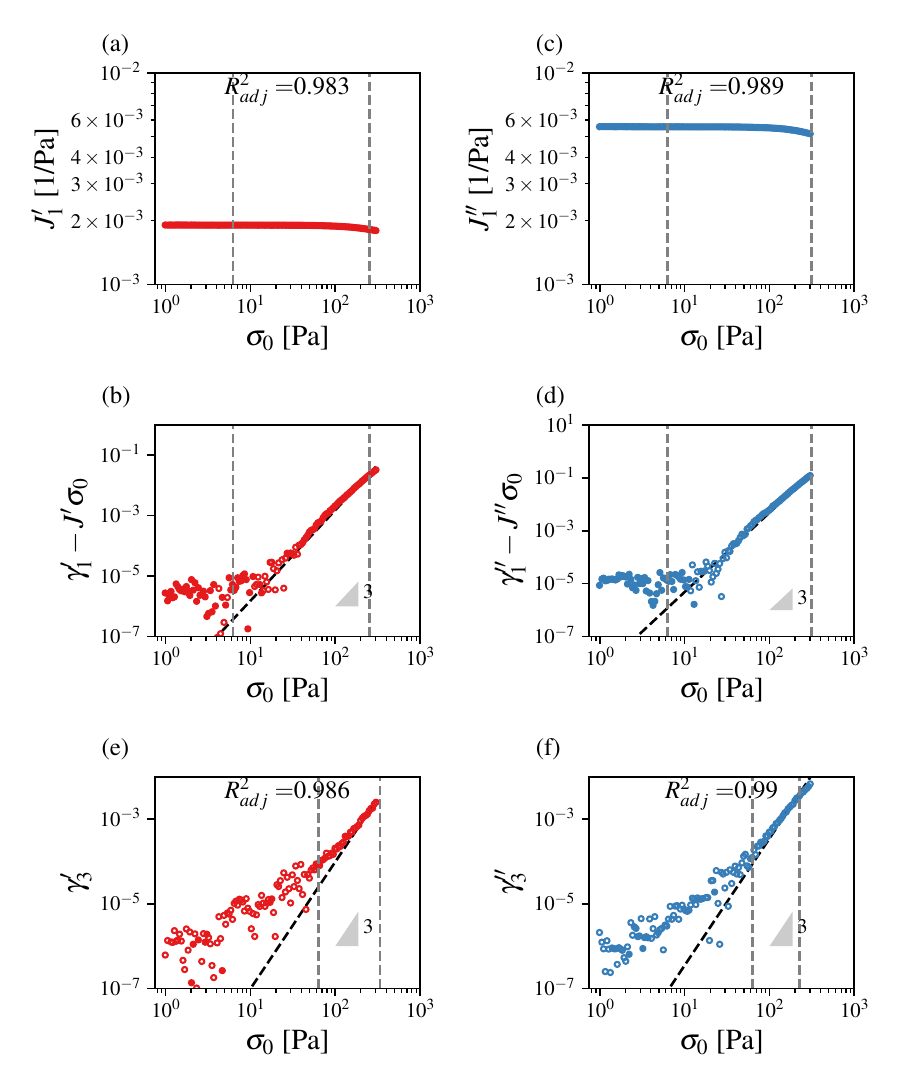}
\caption{The harmonics and fits for $\omega=0.398$ rad/s. Black lines are the fits to data using the MAOStress expansions in Eq. (4). Solid lines represent a positive sign  and dashed lines represent negative sign associated with the magnitude on the log-log scale. The gray vertical dashed lines represent the minimum and maximum stress amplitudes of the fit region that were chosen to fit the MAOStress expansion in Eq. (4).}
\end{figure}

\begin{figure}[h!] 
\centering
\includegraphics{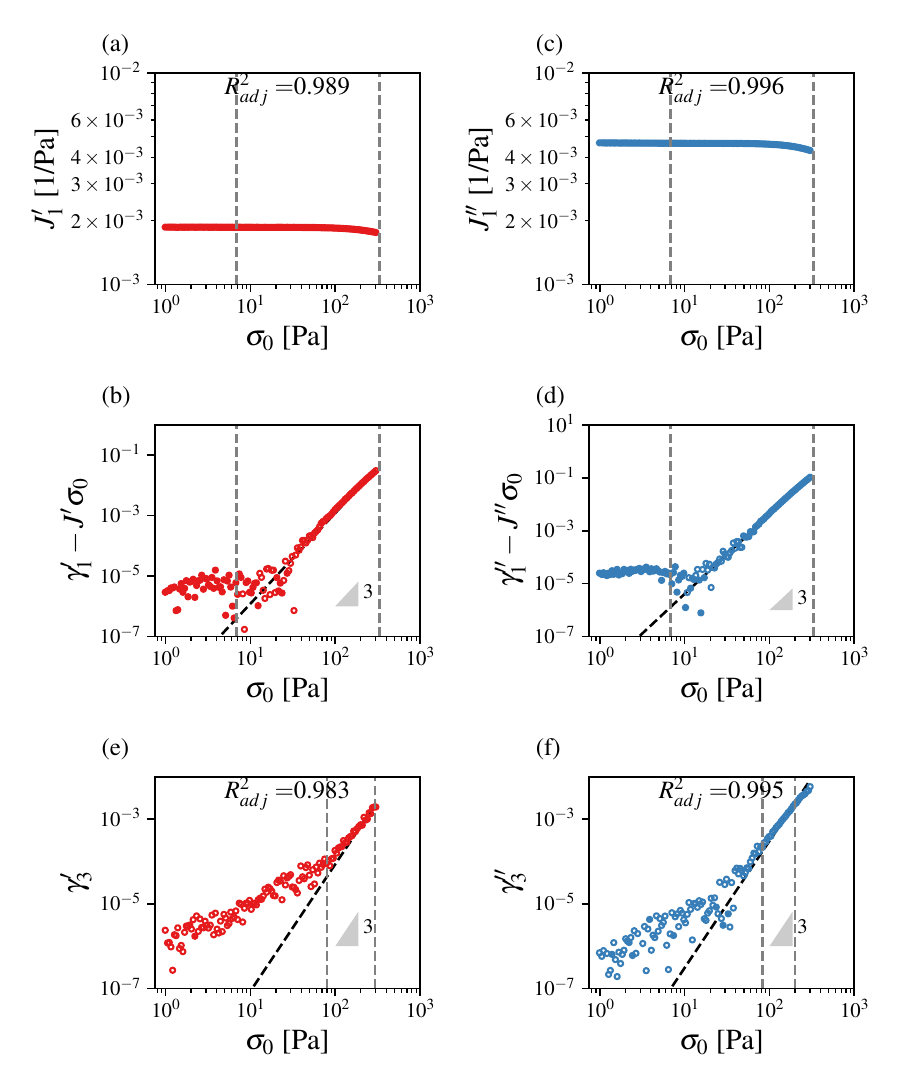}
\caption{The harmonics and fits for $\omega=0.5$ rad/s. Black lines are the fits to data using the MAOStress expansions in Eq. (4). Solid lines represent a positive sign  and dashed lines represent negative sign associated with the magnitude on the log-log scale. The gray vertical dashed lines represent the minimum and maximum stress amplitudes of the fit region that were chosen to fit the MAOStress expansion in Eq. (4).}
\end{figure}

\begin{figure}[h!] 
\centering
\includegraphics{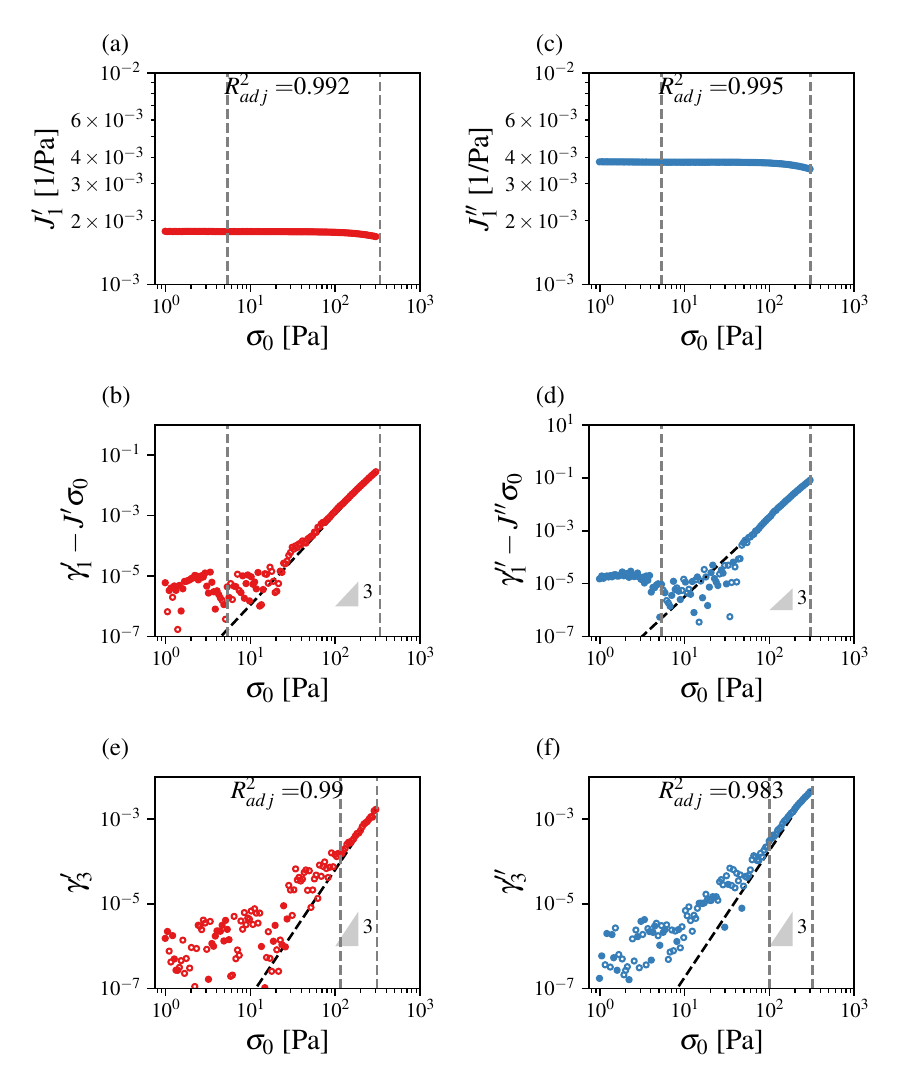}
\caption{The harmonics and fits for $\omega=0.631$ rad/s. Black lines are the fits to data using the MAOStress expansions in Eq. (4). Solid lines represent a positive sign  and dashed lines represent negative sign associated with the magnitude on the log-log scale. The gray vertical dashed lines represent the minimum and maximum stress amplitudes of the fit region that were chosen to fit the MAOStress expansion in Eq. (4).}
\end{figure}

\begin{figure}[h!] 
\centering
\includegraphics{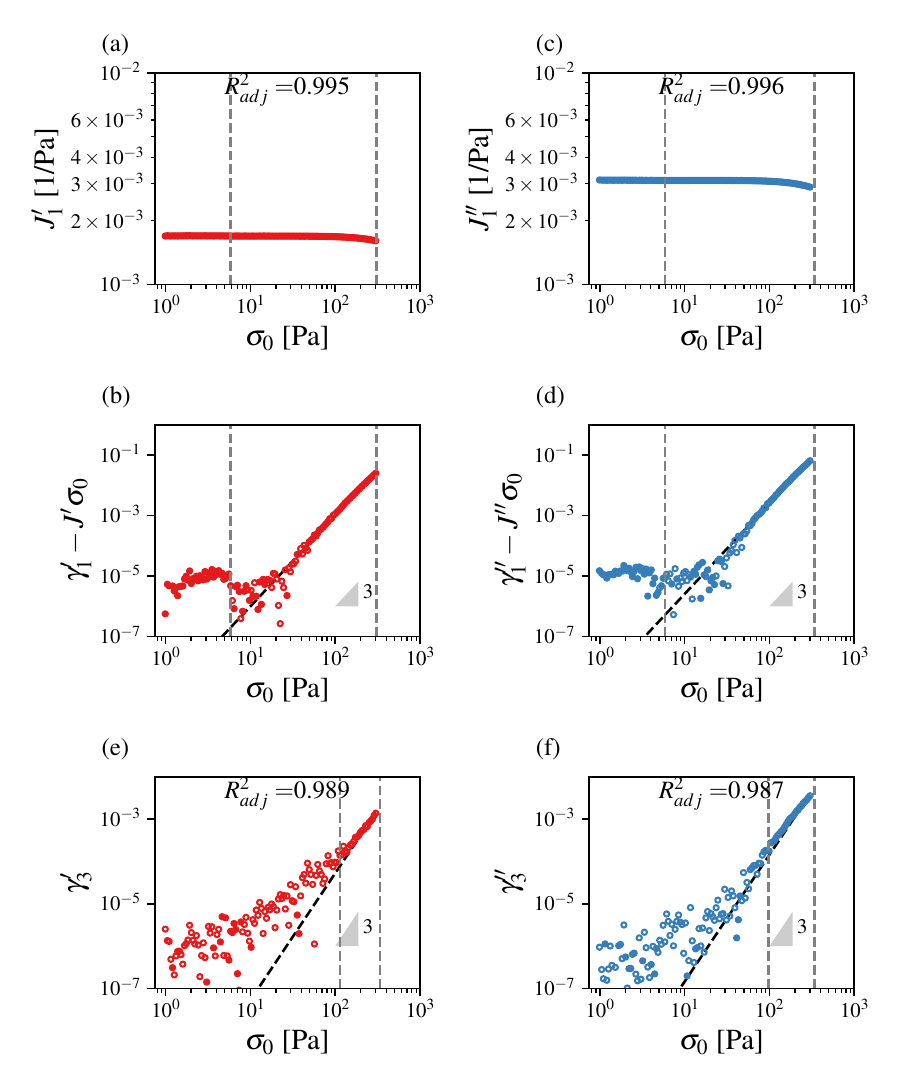}
\caption{The harmonics and fits for $\omega=0.794$ rad/s. Black lines are the fits to data using the MAOStress expansions in Eq. (4). Solid lines represent a positive sign  and dashed lines represent negative sign associated with the magnitude on the log-log scale. The gray vertical dashed lines represent the minimum and maximum stress amplitudes of the fit region that were chosen to fit the MAOStress expansion in Eq. (4).}
\end{figure}

\begin{figure}[h!] 
\centering
\includegraphics{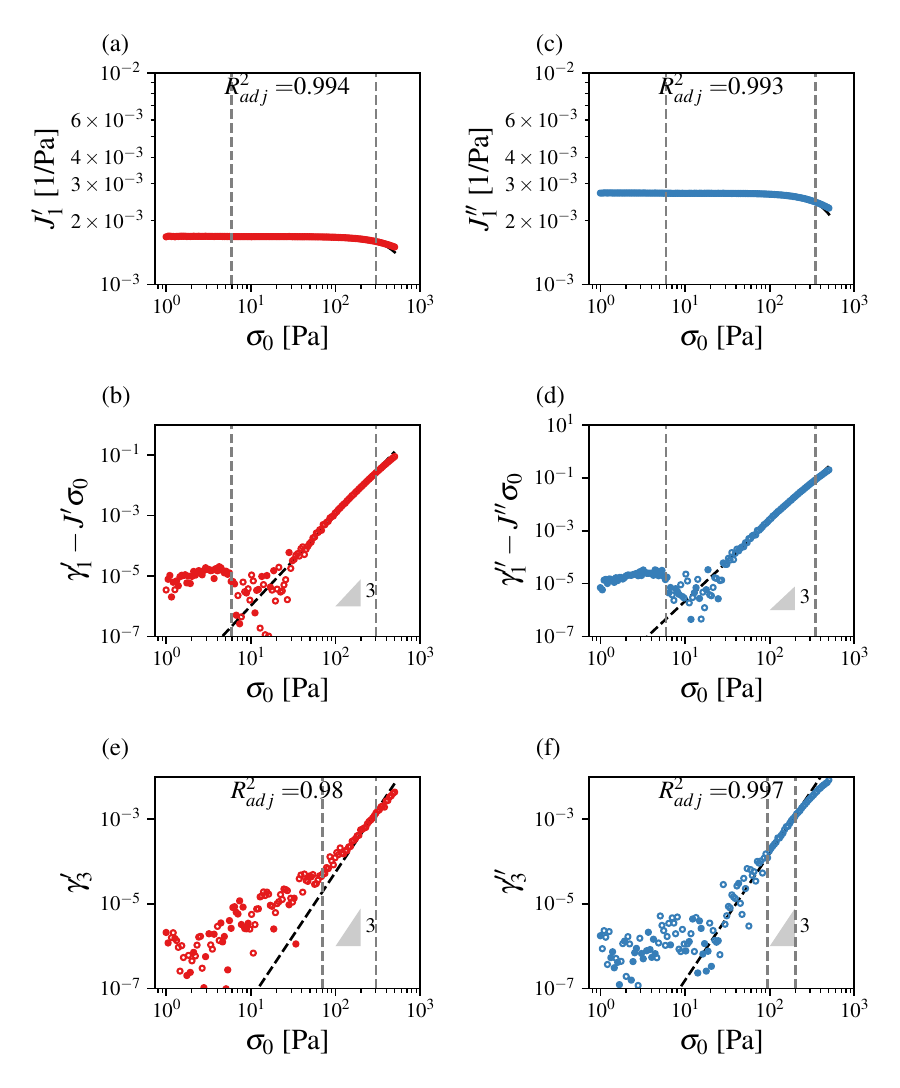}
\caption{The harmonics and fits for $\omega=1.0$ rad/s. Black lines are the fits to data using the MAOStress expansions in Eq. (4). Solid lines represent a positive sign  and dashed lines represent negative sign associated with the magnitude on the log-log scale. The gray vertical dashed lines represent the minimum and maximum stress amplitudes of the fit region that were chosen to fit the MAOStress expansion in Eq. (4).}
\end{figure}

\begin{figure}[h!] 
\centering
\includegraphics{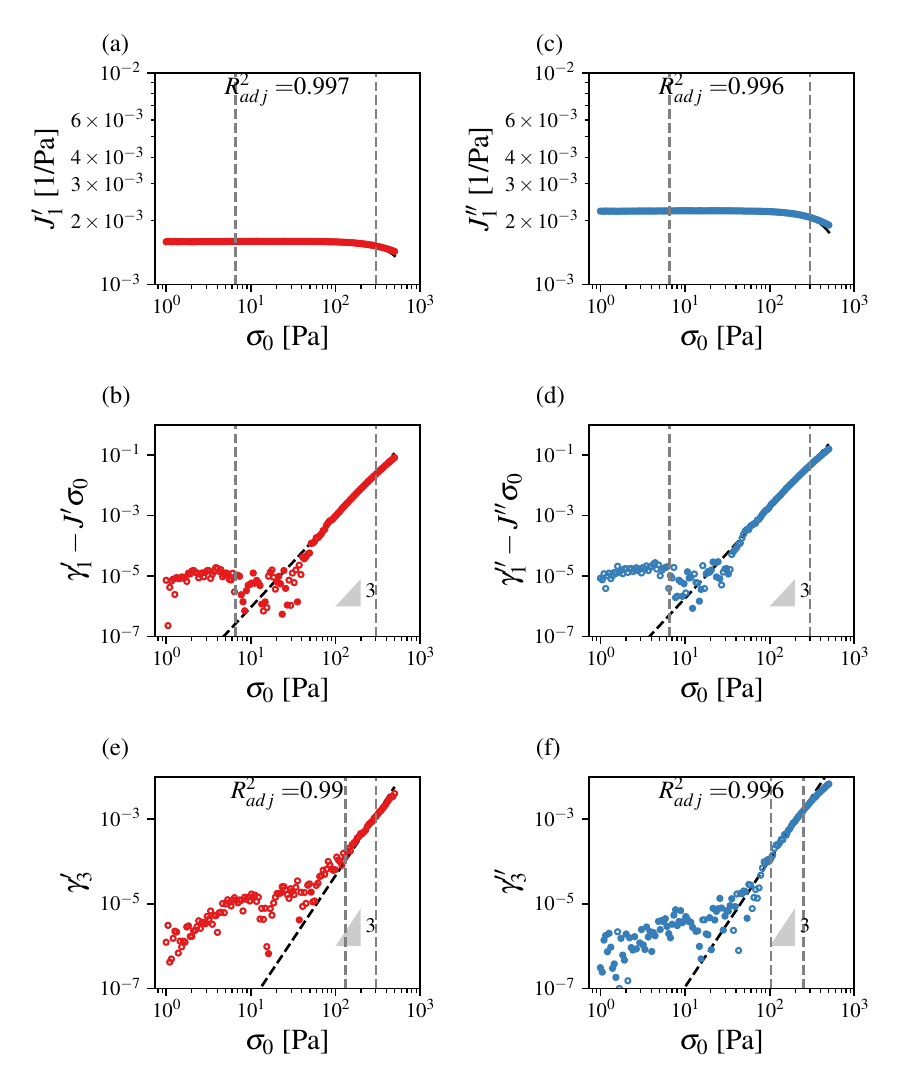}
\caption{The harmonics and fits for $\omega=1.26$ rad/s. Black lines are the fits to data using the MAOStress expansions in Eq. (4). Solid lines represent a positive sign  and dashed lines represent negative sign associated with the magnitude on the log-log scale. The gray vertical dashed lines represent the minimum and maximum stress amplitudes of the fit region that were chosen to fit the MAOStress expansion in Eq. (4).}
\end{figure}

\begin{figure}[h!] 
\centering
\includegraphics{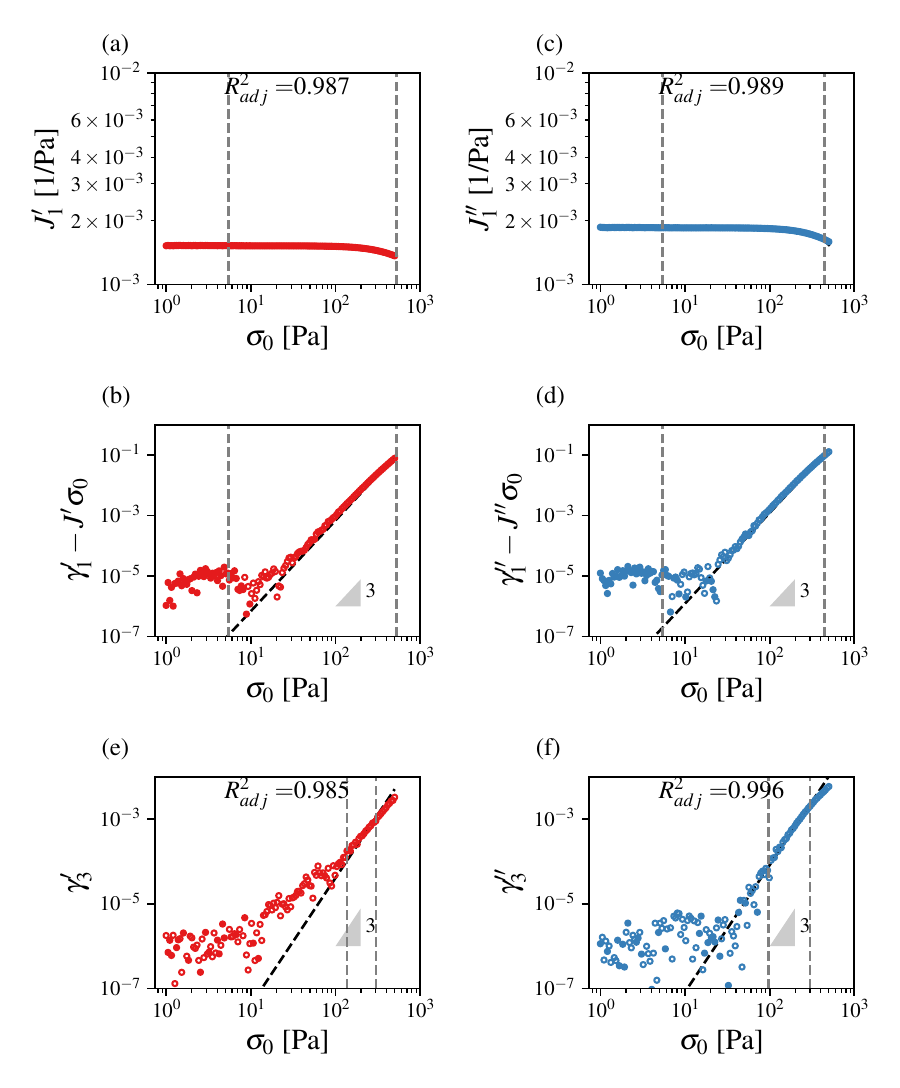}
\caption{The harmonics and fits for $\omega=1.58$ rad/s. Black lines are the fits to data using the MAOStress expansions in Eq. (4). Solid lines represent a positive sign  and dashed lines represent negative sign associated with the magnitude on the log-log scale. The gray vertical dashed lines represent the minimum and maximum stress amplitudes of the fit region that were chosen to fit the MAOStress expansion in Eq. (4).}
\end{figure}

\begin{figure}[h!] 
\centering
\includegraphics{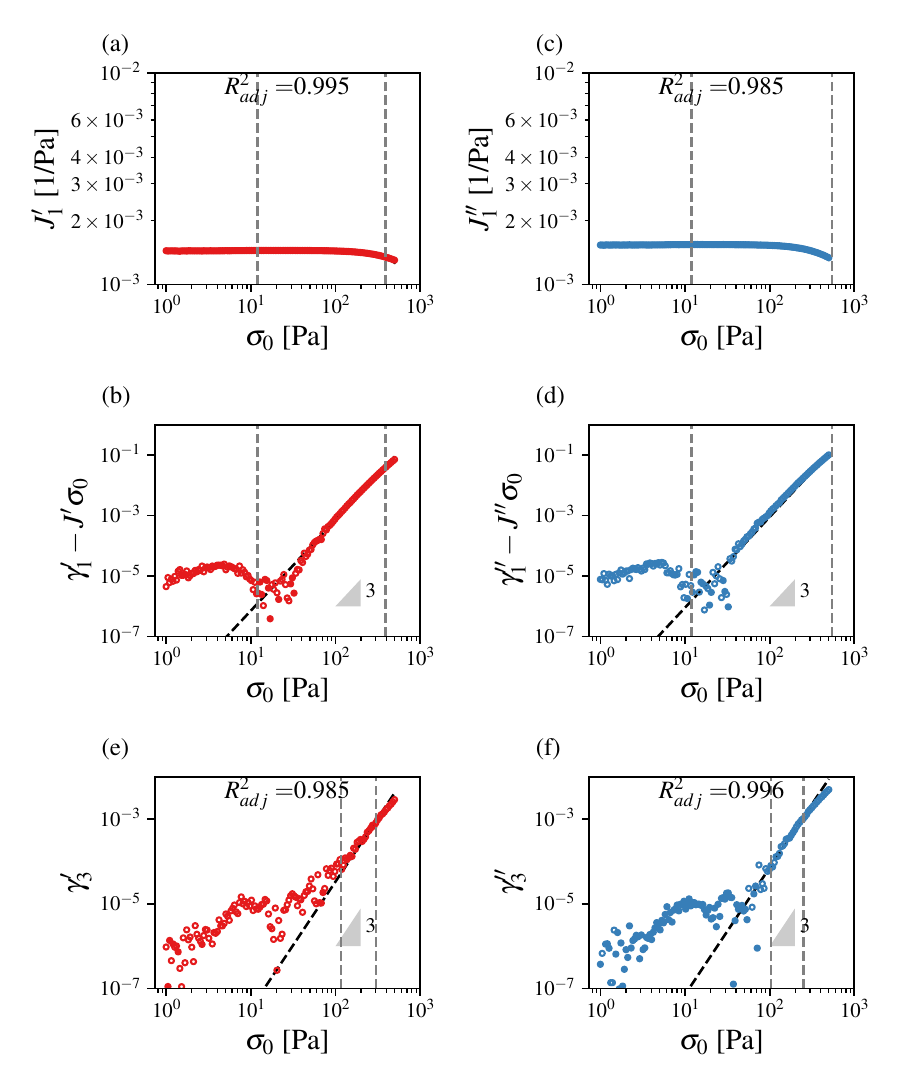}
\caption{The harmonics and fits for $\omega=2.0$ rad/s. Black lines are the fits to data using the MAOStress expansions in Eq. (4). Solid lines represent a positive sign  and dashed lines represent negative sign associated with the magnitude on the log-log scale. The gray vertical dashed lines represent the minimum and maximum stress amplitudes of the fit region that were chosen to fit the MAOStress expansion in Eq. (4).}
\end{figure}

\begin{figure}[h!] 
\centering
\includegraphics{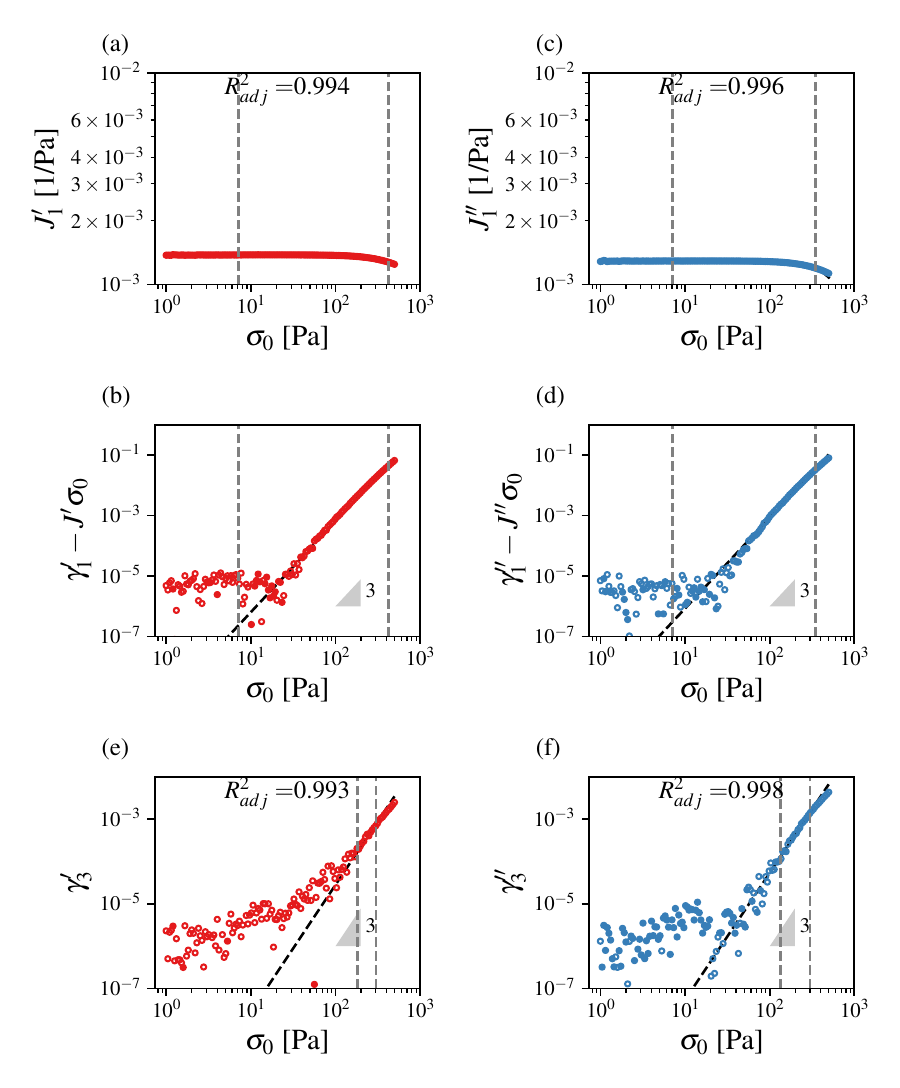}
\caption{The harmonics and fits for $\omega=2.51$ rad/s. Black lines are the fits to data using the MAOStress expansions in Eq. (4). Solid lines represent a positive sign  and dashed lines represent negative sign associated with the magnitude on the log-log scale. The gray vertical dashed lines represent the minimum and maximum stress amplitudes of the fit region that were chosen to fit the MAOStress expansion in Eq. (4).}
\end{figure}

\begin{figure}[h!] 
\centering
\includegraphics{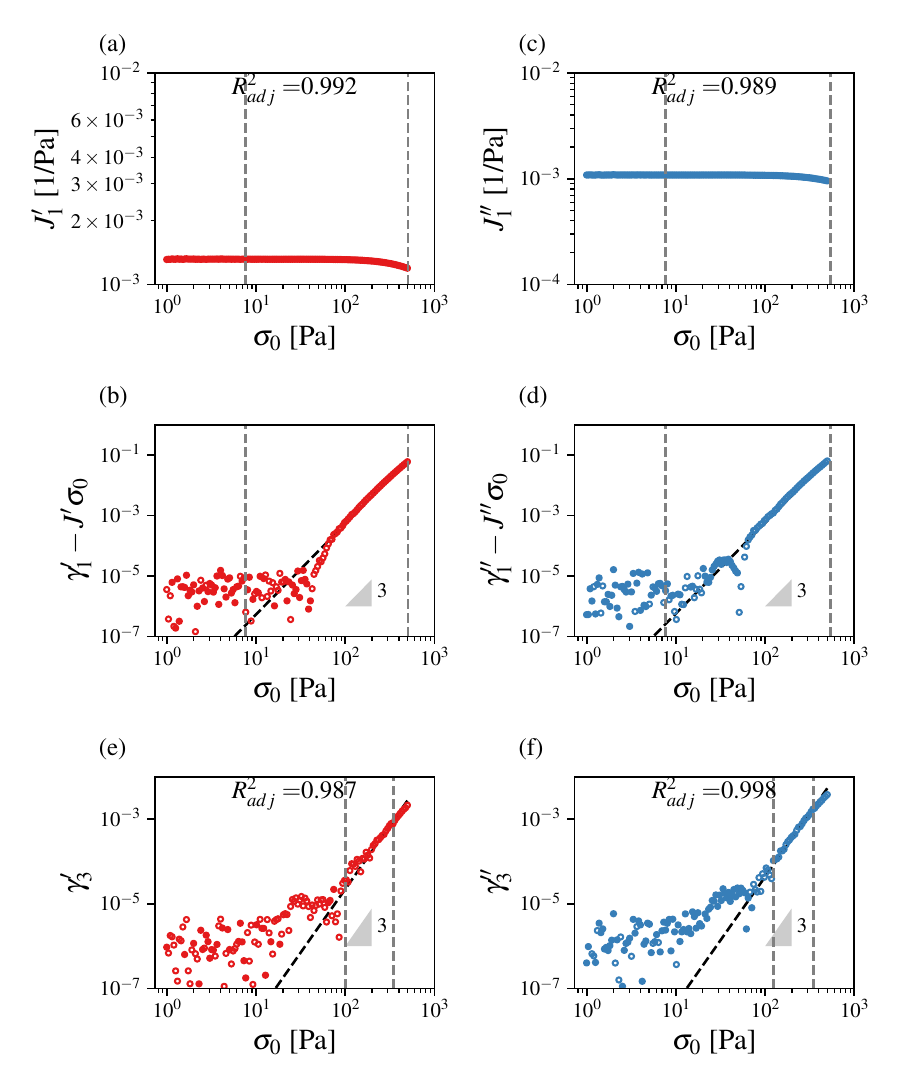}
\caption{The harmonics and fits for $\omega=3.16$ rad/s. Black lines are the fits to data using the MAOStress expansions in Eq. (4). Solid lines represent a positive sign  and dashed lines represent negative sign associated with the magnitude on the log-log scale. The gray vertical dashed lines represent the minimum and maximum stress amplitudes of the fit region that were chosen to fit the MAOStress expansion in Eq. (4).}
\end{figure}

\begin{figure}[h!] 
\centering
\includegraphics{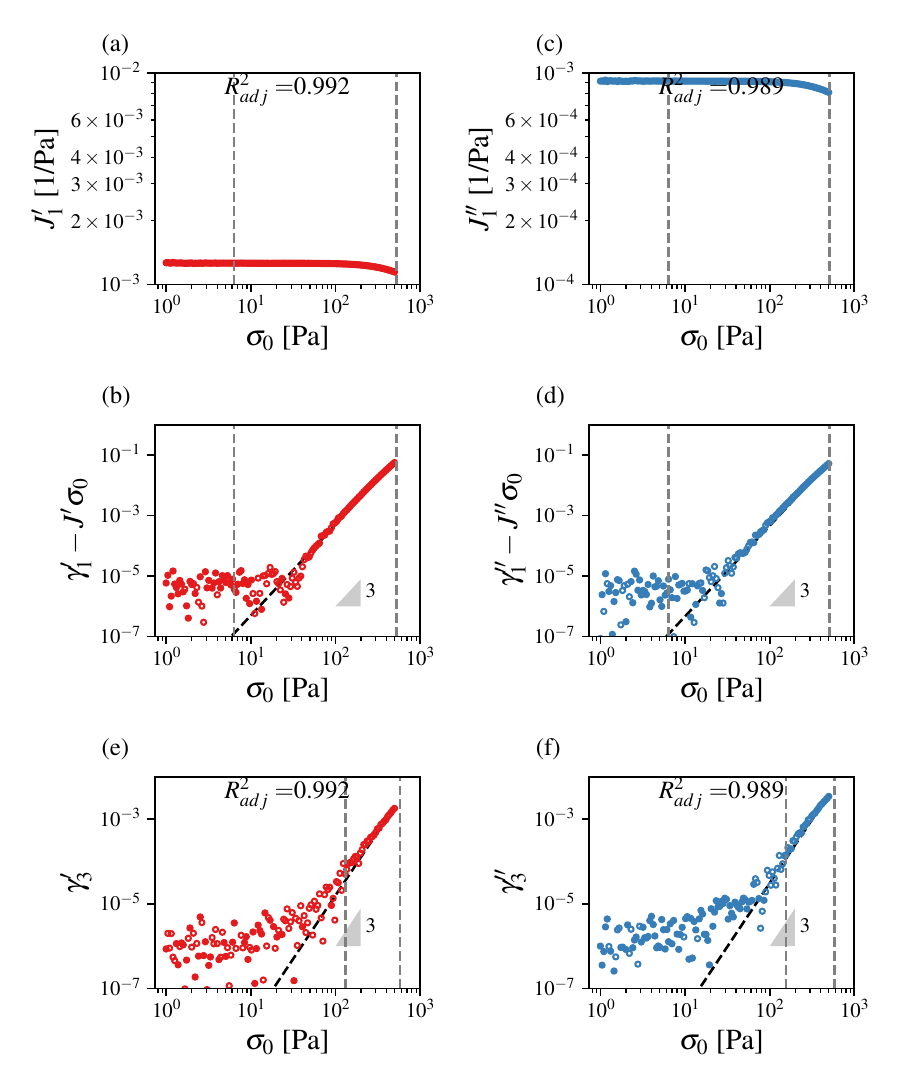}
\caption{The harmonics and fits for $\omega=3.98$ rad/s. Black lines are the fits to data using the MAOStress expansions in Eq. (4). Solid lines represent a positive sign  and dashed lines represent negative sign associated with the magnitude on the log-log scale. The gray vertical dashed lines represent the minimum and maximum stress amplitudes of the fit region that were chosen to fit the MAOStress expansion in Eq. (4).}
\end{figure}

\begin{figure}[h!] 
\centering
\includegraphics{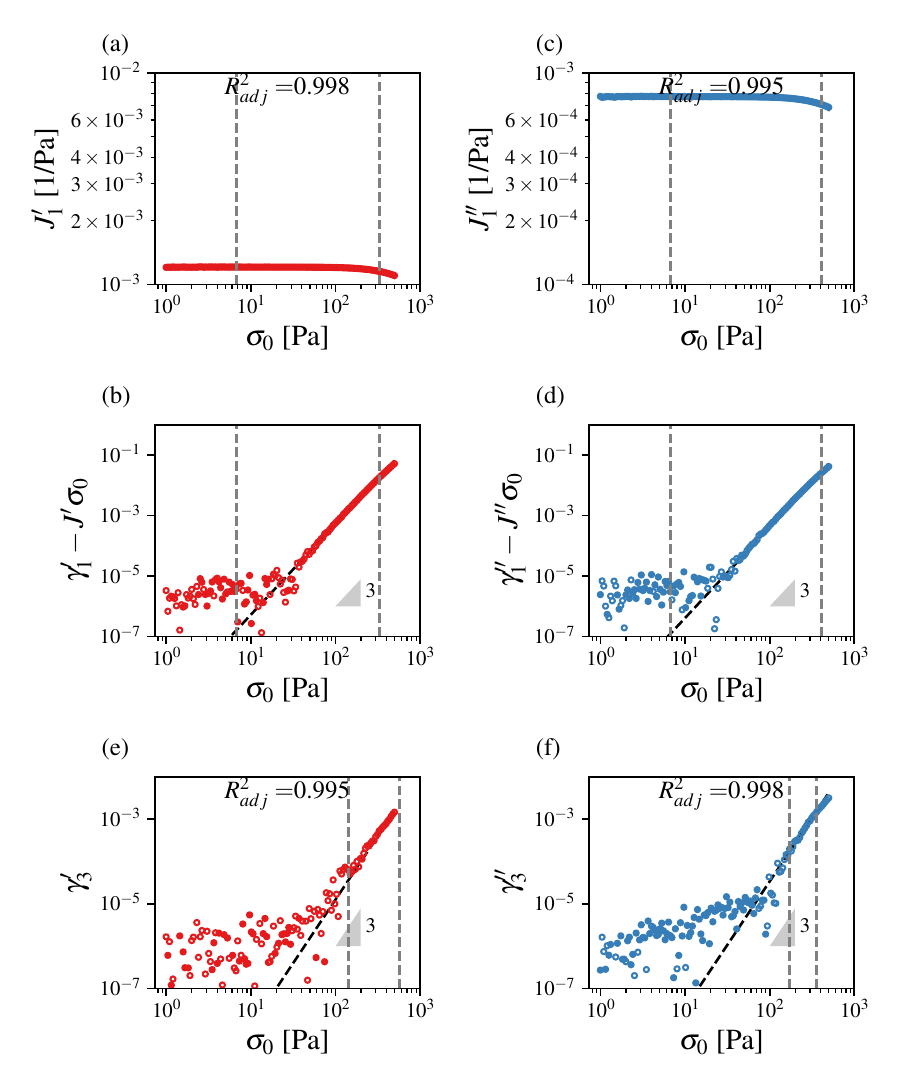}
\caption{The harmonics and fits for $\omega=5.01$ rad/s. Black lines are the fits to data using the MAOStress expansions in Eq. (4). Solid lines represent a positive sign  and dashed lines represent negative sign associated with the magnitude on the log-log scale. The gray vertical dashed lines represent the minimum and maximum stress amplitudes of the fit region that were chosen to fit the MAOStress expansion in Eq. (4).}
\end{figure}

\begin{figure}[h!] 
\centering
\includegraphics{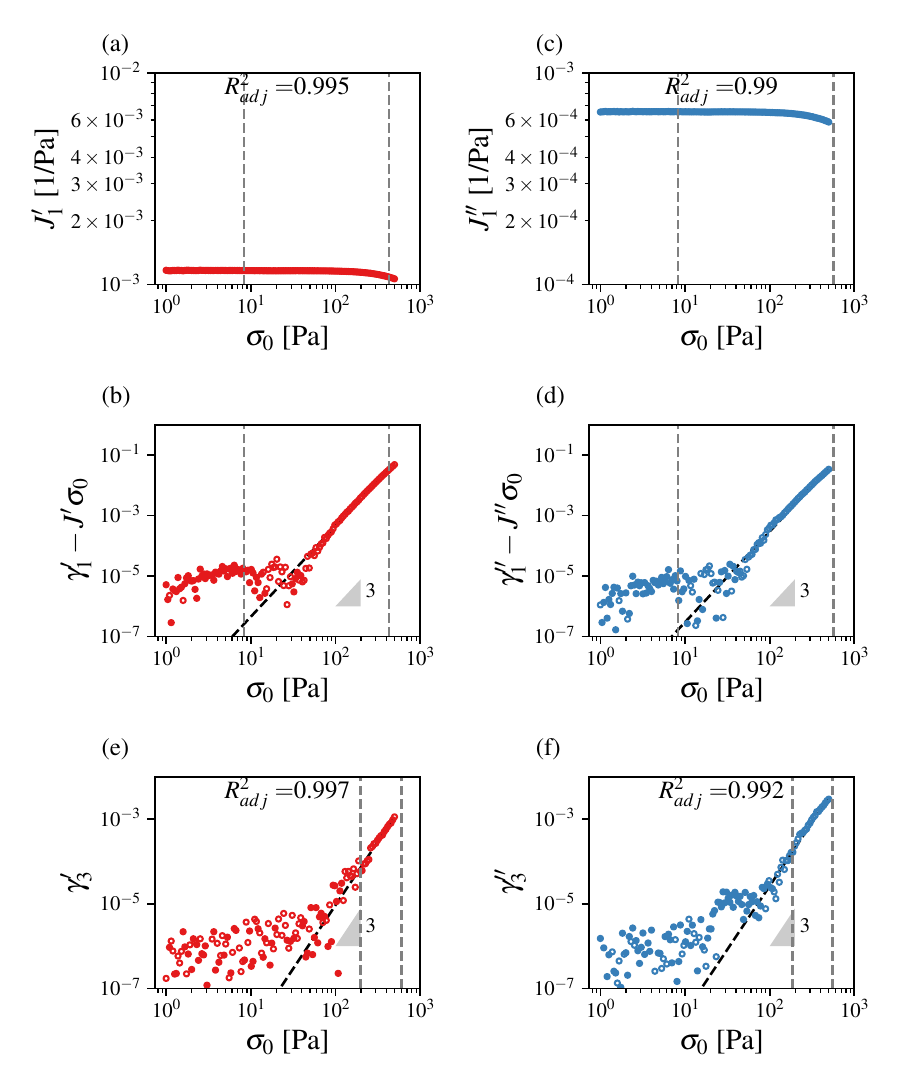}
\caption{The harmonics and fits for $\omega=6.31$ rad/s. Black lines are the fits to data using the MAOStress expansions in Eq. (4). Solid lines represent a positive sign  and dashed lines represent negative sign associated with the magnitude on the log-log scale. The gray vertical dashed lines represent the minimum and maximum stress amplitudes of the fit region that were chosen to fit the MAOStress expansion in Eq. (4).}
\end{figure}

\begin{figure}[h!] 
\centering
\includegraphics{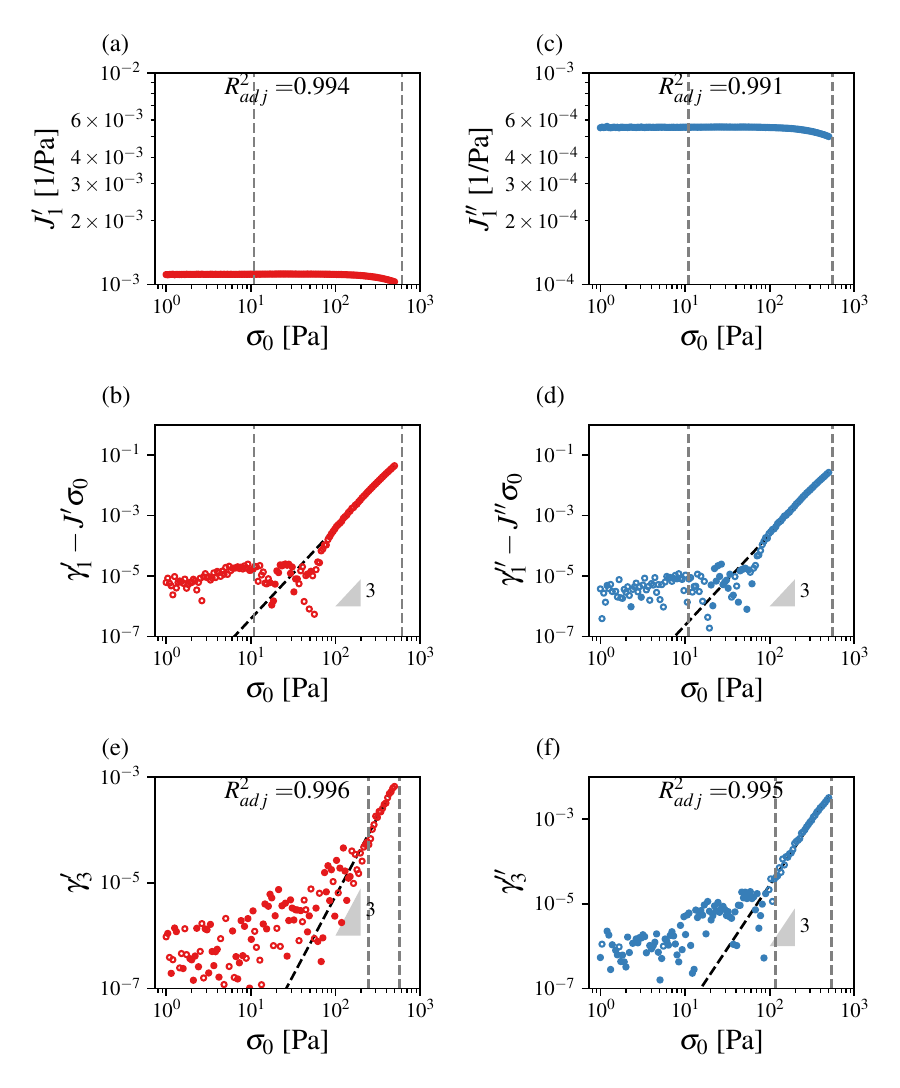}
\caption{The harmonics and fits for $\omega=7.94$ rad/s. Black lines are the fits to data using the MAOStress expansions in Eq. (4). Solid lines represent a positive sign  and dashed lines represent negative sign associated with the magnitude on the log-log scale. The gray vertical dashed lines represent the minimum and maximum stress amplitudes of the fit region that were chosen to fit the MAOStress expansion in Eq. (4).}
\end{figure}

\begin{figure}[h!] 
\centering
\includegraphics{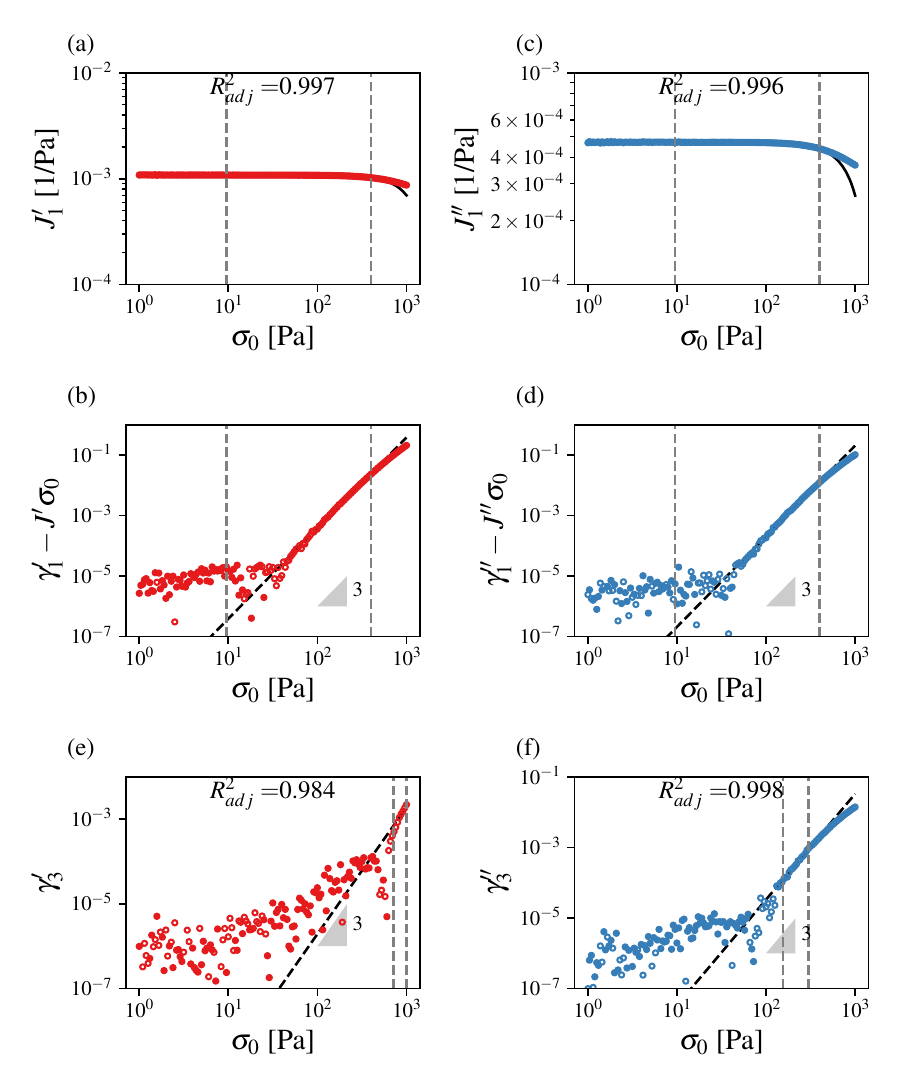}
\caption{The harmonics and fits for $\omega=10.0$ rad/s. Black lines are the fits to data using the MAOStress expansions in Eq. (4). Solid lines represent a positive sign  and dashed lines represent negative sign associated with the magnitude on the log-log scale. The gray vertical dashed lines represent the minimum and maximum stress amplitudes of the fit region that were chosen to fit the MAOStress expansion in Eq. (4).}
\end{figure}

\begin{figure}[h!] 
\centering
\includegraphics{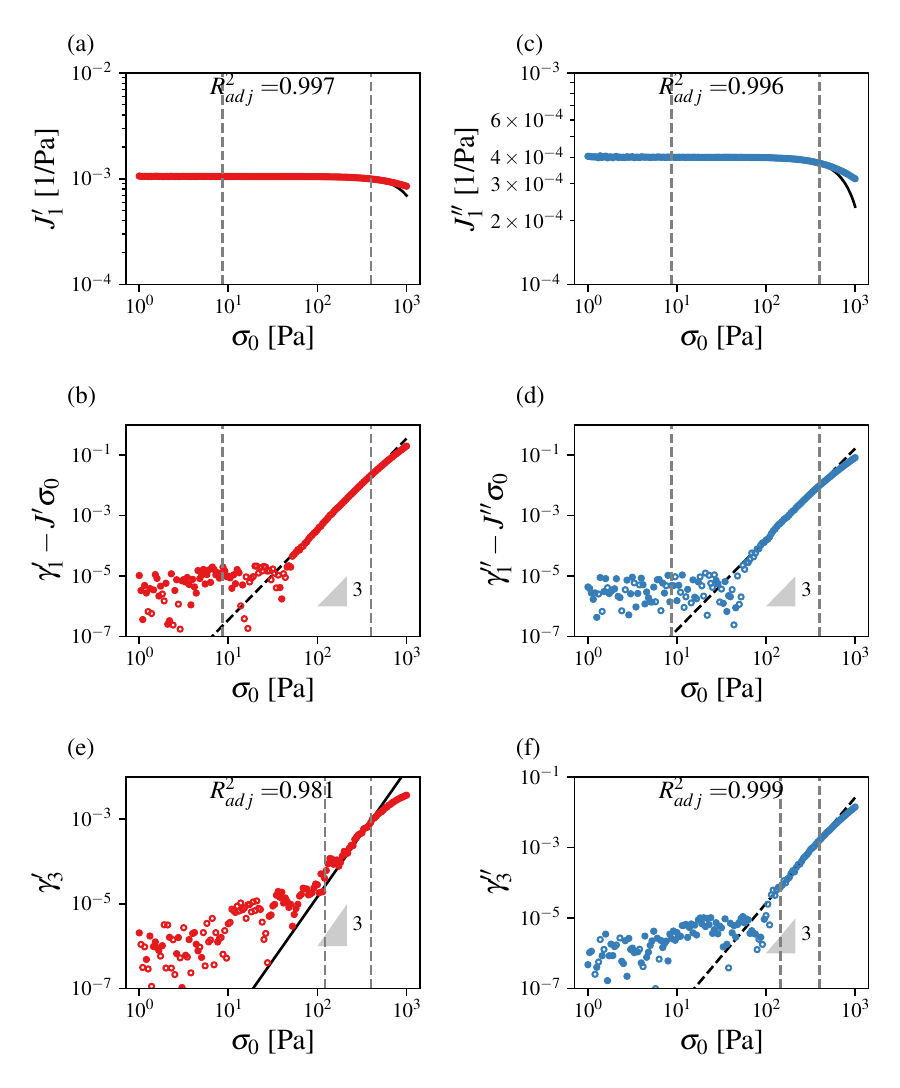}
\caption{The harmonics and fits for $\omega=12.6$ rad/s. Black lines are the fits to data using the MAOStress expansions in Eq. (4). Solid lines represent a positive sign  and dashed lines represent negative sign associated with the magnitude on the log-log scale. The gray vertical dashed lines represent the minimum and maximum stress amplitudes of the fit region that were chosen to fit the MAOStress expansion in Eq. (4).}
\end{figure}

\begin{figure}[h!] 
\centering
\includegraphics{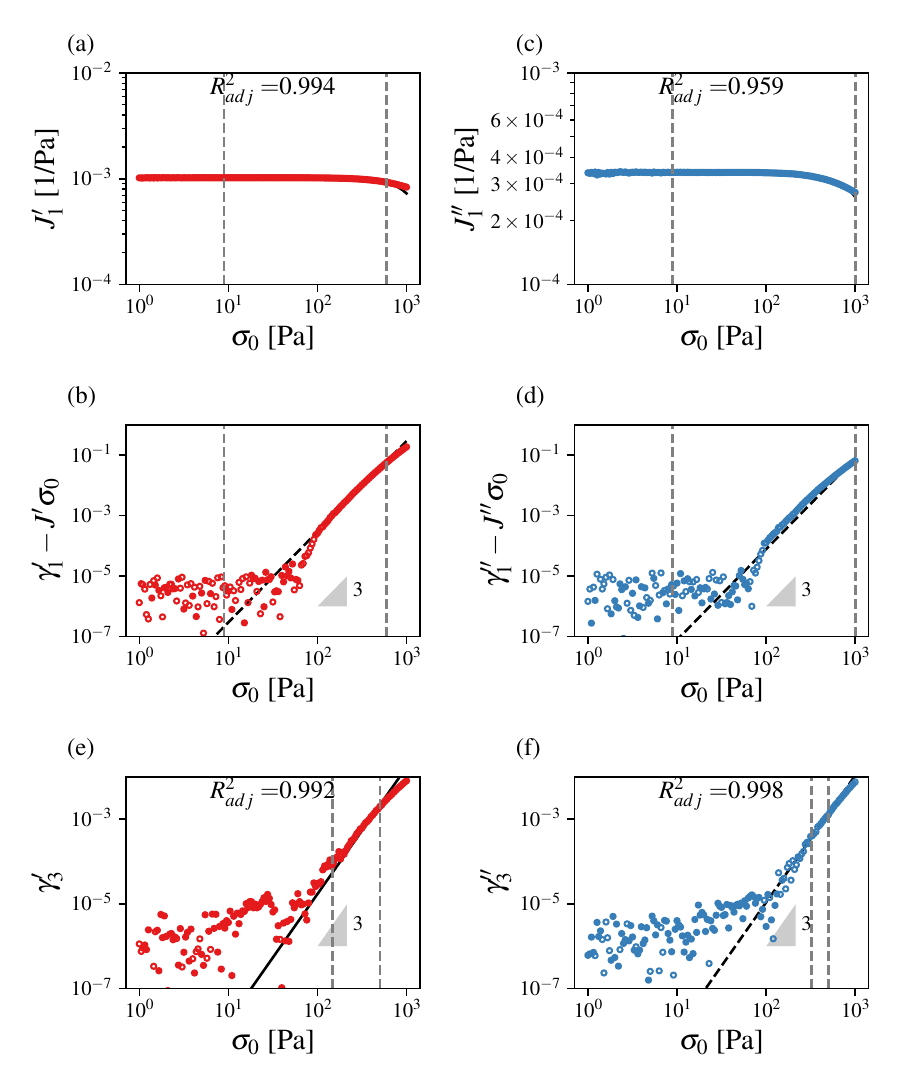}
\caption{The harmonics and fits for $\omega=15.8$ rad/s. Black lines are the fits to data using the MAOStress expansions in Eq. (4). Solid lines represent a positive sign  and dashed lines represent negative sign associated with the magnitude on the log-log scale. The gray vertical dashed lines represent the minimum and maximum stress amplitudes of the fit region that were chosen to fit the MAOStress expansion in Eq. (4).}
\end{figure}

\begin{figure}[h!] 
\centering
\includegraphics{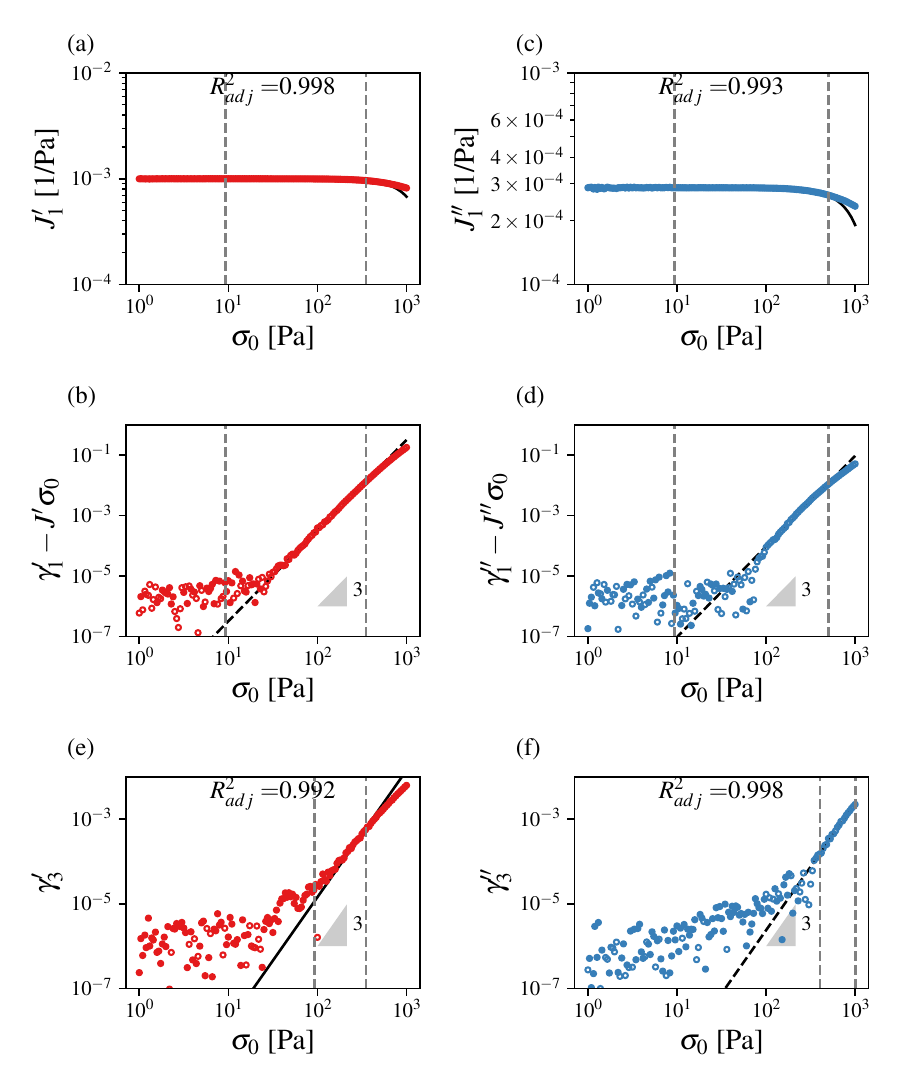}
\caption{The harmonics and fits for $\omega=20.0$ rad/s. Black lines are the fits to data using the MAOStress expansions in Eq. (4). Solid lines represent a positive sign  and dashed lines represent negative sign associated with the magnitude on the log-log scale. The gray vertical dashed lines represent the minimum and maximum stress amplitudes of the fit region that were chosen to fit the MAOStress expansion in Eq. (4).}
\end{figure}

\begin{figure}[h!] 
\centering
\includegraphics{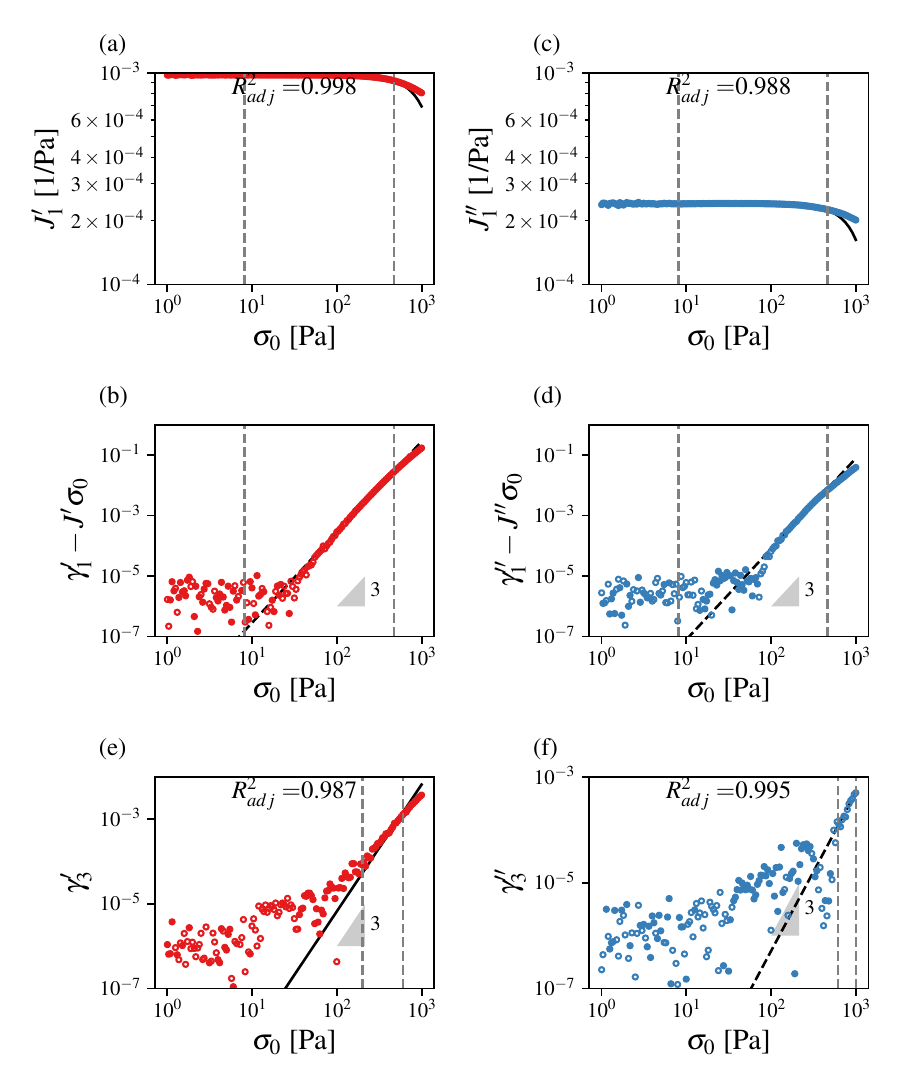}
\caption{The harmonics and fits for $\omega=25.1$ rad/s. Black lines are the fits to data using the MAOStress expansions in Eq. (4). Solid lines represent a positive sign  and dashed lines represent negative sign associated with the magnitude on the log-log scale. The gray vertical dashed lines represent the minimum and maximum stress amplitudes of the fit region that were chosen to fit the MAOStress expansion in Eq. (4).}
\end{figure}

\begin{figure}[h!] 
\centering
\includegraphics{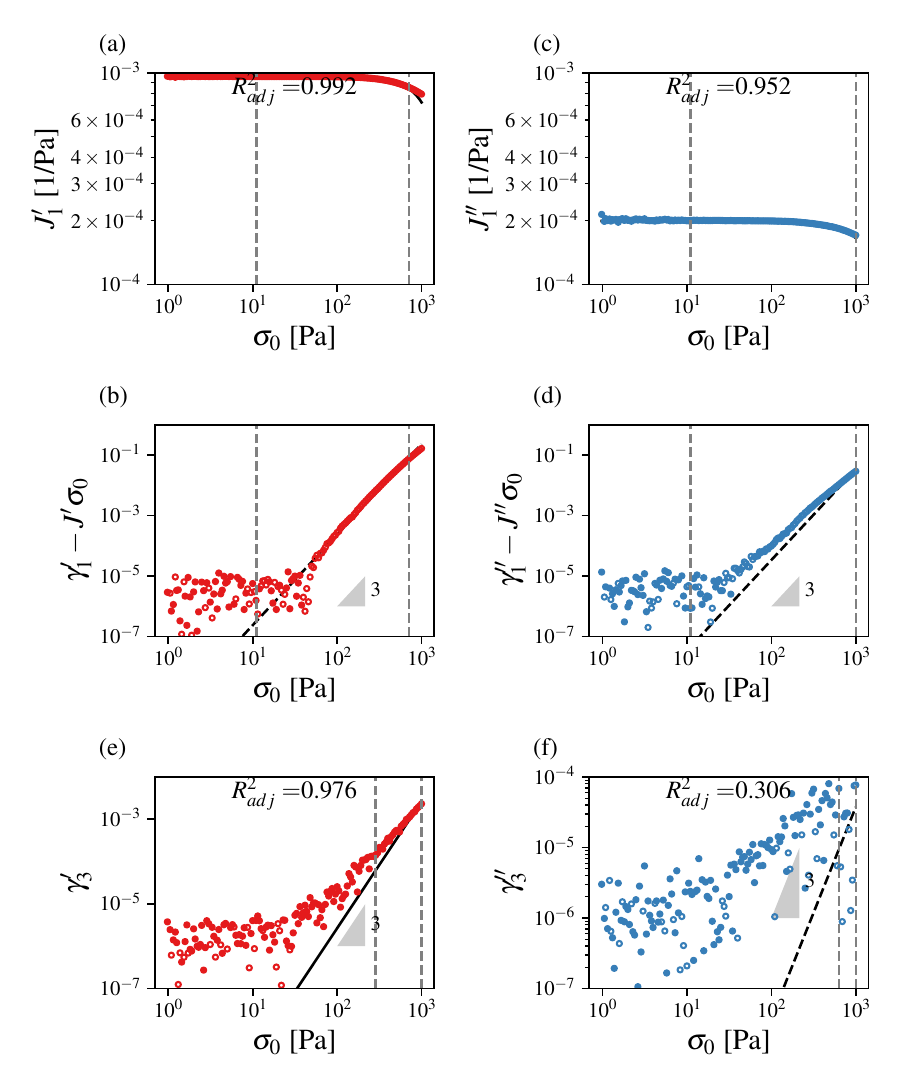}
\caption{The harmonics and fits for $\omega=31.6$ rad/s. Black lines are the fits to data using the MAOStress expansions in Eq. (4). Solid lines represent a positive sign  and dashed lines represent negative sign associated with the magnitude on the log-log scale. The gray vertical dashed lines represent the minimum and maximum stress amplitudes of the fit region that were chosen to fit the MAOStress expansion in Eq. (4).}
\end{figure}

\begin{figure}[h!] 
\centering
\includegraphics{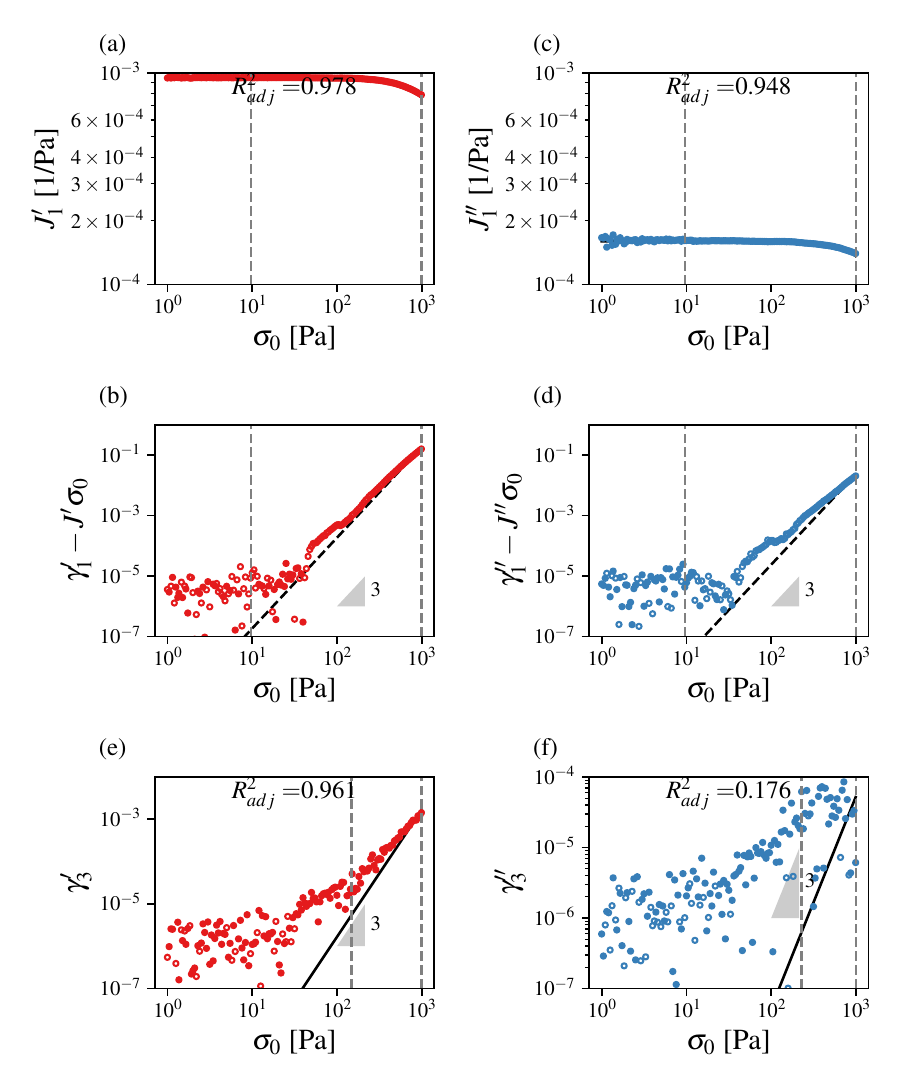}
\caption{The harmonics and fits for $\omega=39.8$ rad/s. Black lines are the fits to data using the MAOStress expansions in Eq. (4). Solid lines represent a positive sign  and dashed lines represent negative sign associated with the magnitude on the log-log scale. The gray vertical dashed lines represent the minimum and maximum stress amplitudes of the fit region that were chosen to fit the MAOStress expansion in Eq. (4).}
\end{figure}

\begin{figure}[h!] 
\centering
\includegraphics{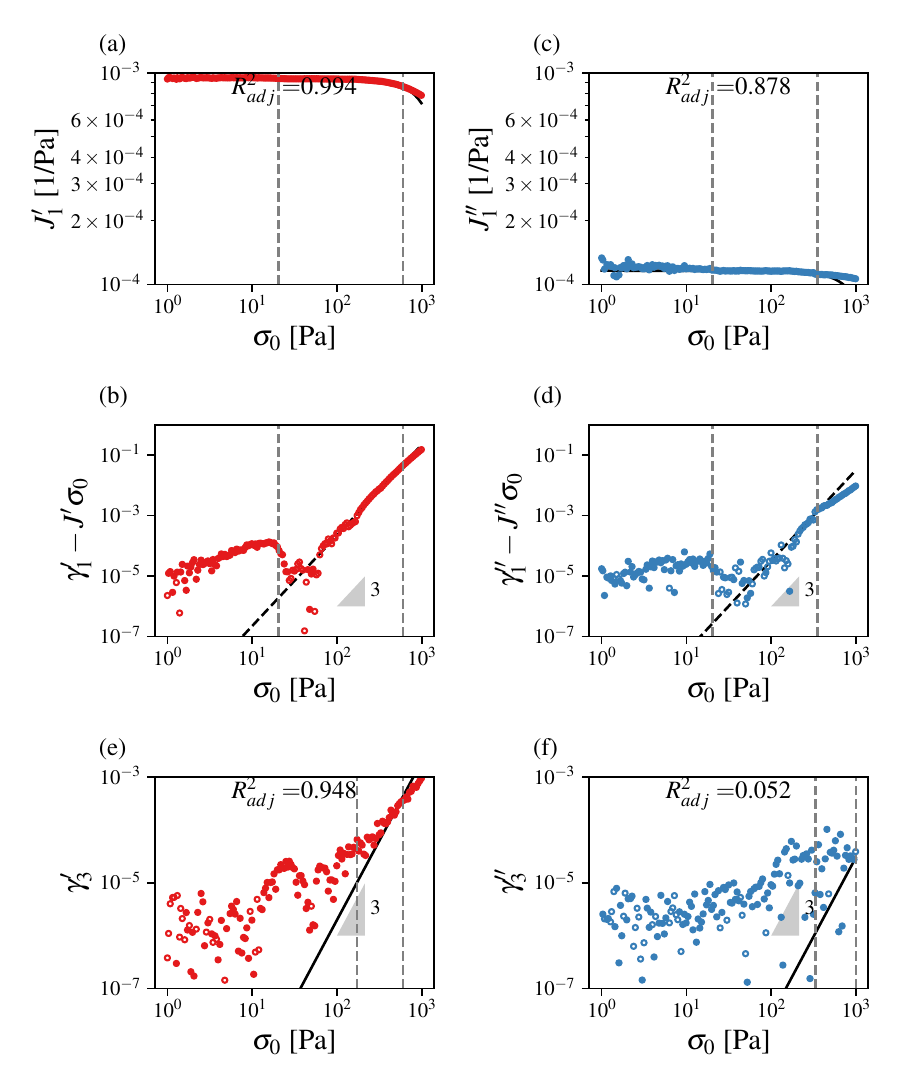}
\caption{The harmonics and fits for $\omega=50.1$ rad/s. Black lines are the fits to data using the MAOStress expansions in Eq. (4). Solid lines represent a positive sign  and dashed lines represent negative sign associated with the magnitude on the log-log scale. The gray vertical dashed lines represent the minimum and maximum stress amplitudes of the fit region that were chosen to fit the MAOStress expansion in Eq. (4).}
\end{figure}

\begin{figure}[h!] 
\centering
\includegraphics{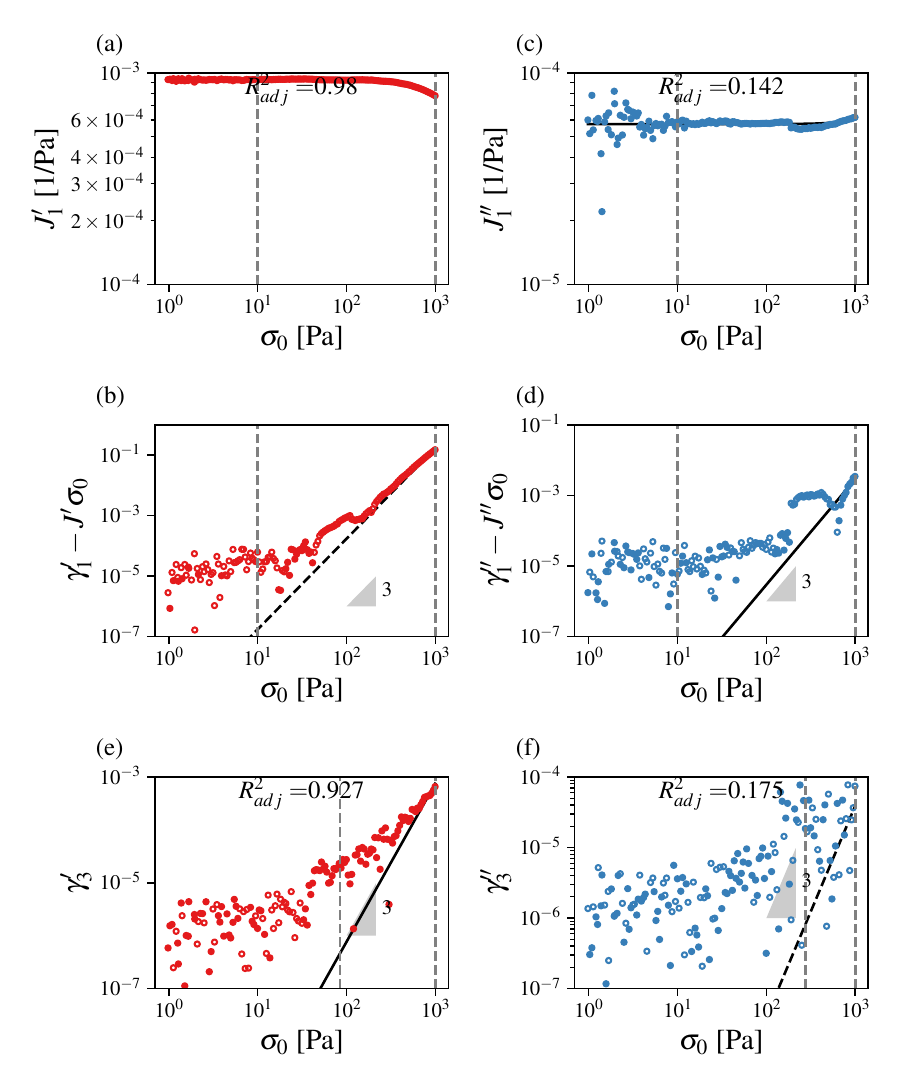}
\caption{The harmonics and fits for $\omega=63.1$ rad/s. Black lines are the fits to data using the MAOStress expansions in Eq. (4). Solid lines represent a positive sign  and dashed lines represent negative sign associated with the magnitude on the log-log scale. The gray vertical dashed lines represent the minimum and maximum stress amplitudes of the fit region that were chosen to fit the MAOStress expansion in Eq. (4).}
\end{figure}

\begin{figure}[h!] 
\centering
\includegraphics{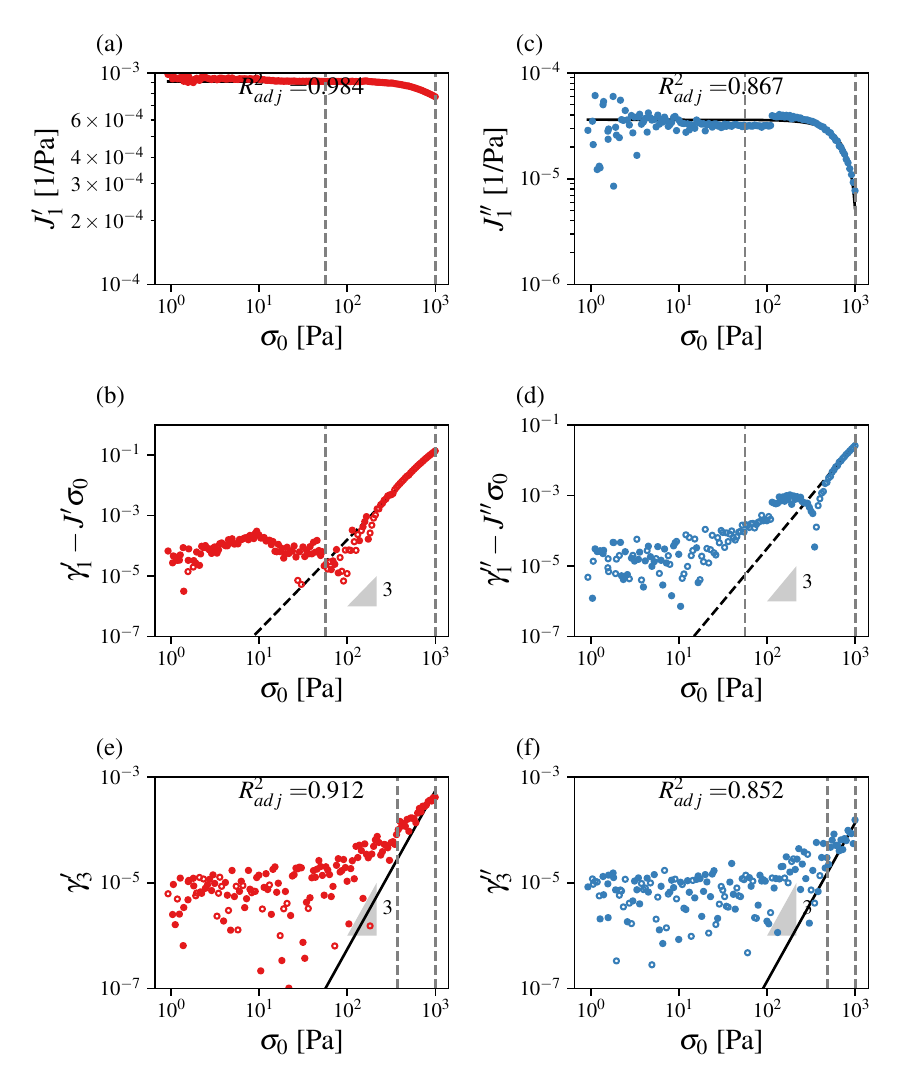}
\caption{The harmonics and fits for $\omega=79.4$ rad/s. Black lines are the fits to data using the MAOStress expansions in Eq. (4). Solid lines represent a positive sign  and dashed lines represent negative sign associated with the magnitude on the log-log scale. The gray vertical dashed lines represent the minimum and maximum stress amplitudes of the fit region that were chosen to fit the MAOStress expansion in Eq. (4).}
\end{figure}

\begin{figure}[h!] 
\centering
\includegraphics{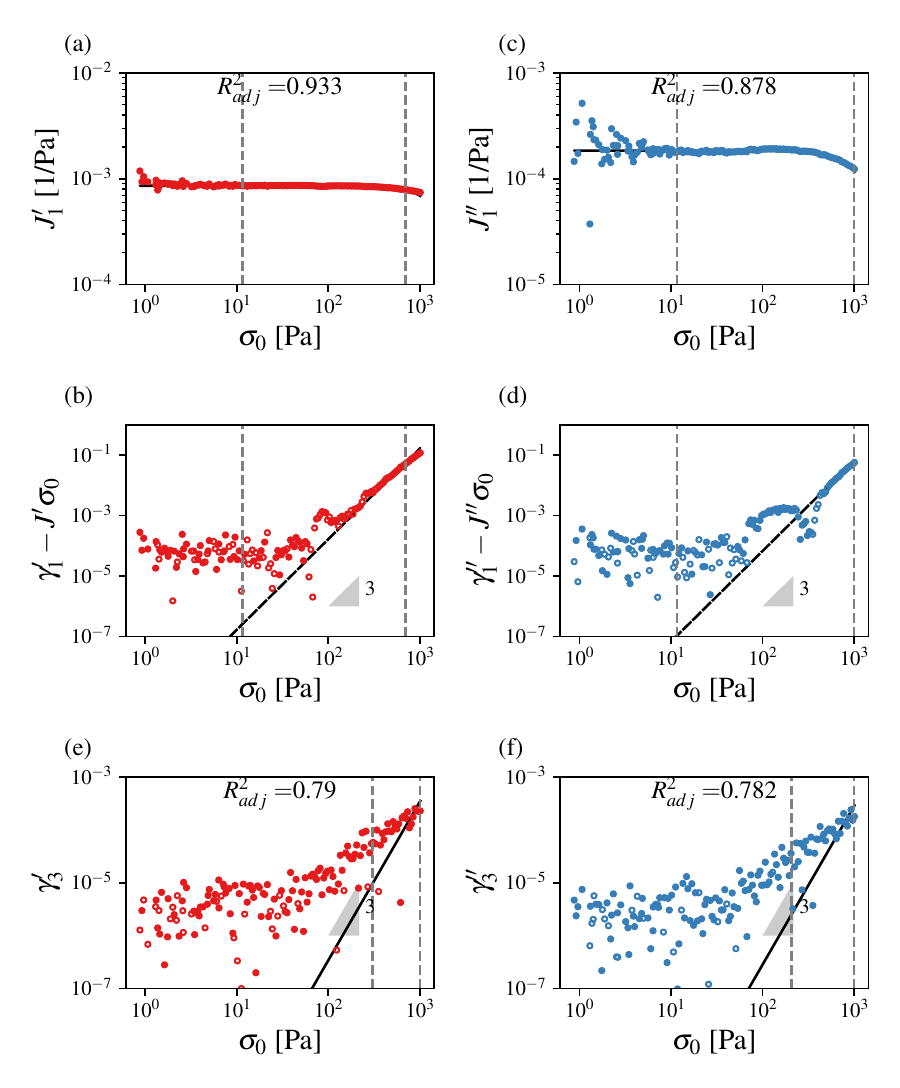}
\caption{The harmonics and fits for $\omega=100.0$ rad/s. Black lines are the fits to data using the MAOStress expansions in Eq. (4). Solid lines represent a positive sign  and dashed lines represent negative sign associated with the magnitude on the log-log scale. The gray vertical dashed lines represent the minimum and maximum stress amplitudes of the fit region that were chosen to fit the MAOStress expansion in Eq. (4).}
\end{figure}
